# Supplementary material for: Optimal enzyme rhythms in cells
Source: arXiv:1602.05167 source file (2022-10-04)
Supplement: Supplementary file 1 [file sec_supplement_optimal_enzyme_rhythms.tex]

\co{ueberlegen: can we know anything about the largest eigenvalue (or its reasons
  by ``synergistic cycles'') by looking at cycles in the matrix? or,
  if we compute the moments of the eigenvalue spectrum from counting
  cycles, can we interpret these moments in any way?

  NOTE: for hermitian matrix A, the largest eigenvalue must as equal or larger than:
  \[
    \gamma_{1(A)} = \min\{ \frac{1}{n}\sum_{ij} a_{ij}, \frac{1}{n} \sum_{i} a_{ii} - \frac{1}{n(n-1) \sum_{i\ne j} a_{ij}}\}
  \]

  ref rachid marsli  (2015) ``Bounds for the smallest and the largest eigenvalue of hermitian matrices'', int j of algebra vol 9 no 8 p 379-394

  stems from Weyl inequalities for n x n hermitian matrices (where i is index of the eigenvector from low to high)

  \[\lambda_{i}(A_{1}+A_{2}) \ge \lambda_{i-j+1}(A_{1}) + \lambda_{j}(A2)\],

  in particular. 
  \[\lambda_{max}(A_{1}+A_{2}) \ge \lambda_{max}(A_{1}) + \lambda_{min}(A2)\],

}

This supplementary text describes metabolic dynamics, example models,
and mathematical derivations in more detail.  Section
\ref{sec:periodicdynamics} shows how periodic perturbations of single
reactions can be described by spectral elasticities; how biochemical
systems respond to small static or periodic perturbations and how
these responses can be computed with the help of response
coefficients; how static, spectral, and periodic response coefficients
are computed; and how periodic changes in transcript and protein
levels are interrelated.  Section \ref{sec:sioptimaladaption}
describes how optimal enzyme profiles in time are predicted.  In
section \ref{sec:SIexamples}, simple example models are
discussed. Section \ref{sec:proofs} contains mathematical proofs and
derivations, as well as a description of the mathematical notation
(with lists of mathematical symbols in Tables \ref{tab:symbols} and
\ref{tab:symbols2}).

\section{Dynamics of metabolic oscillations}
\label{sec:periodicdynamics}

In kinetic metabolic models, static parameter changes are likely to
shift the steady state.  Periodic parameter changes, instead, will
lead to forced oscillations.  These dynamic responses can be computed
in a second-order approximation, as described in this section
\cite{hesc:96,hohe:93,lieb:2005}.

\subsection{Expansion of peridiodic reaction rates}
\label{sec:nonlinear}

Enzymatic rate laws describe reaction rates as functions of substrate,
product, and enzyme levels.  Reaction elasticities are the derivatives
between a reaction rate and variables that directly determine this
rate (via the rate laws, and without considering stationarity).  The
unscaled reaction elasticities of a rate law $\rate_{k}(\cintv,\pv)$,
defined as
\begin{eqnarray}
\epsilonSkm   &=& \frac{\partial  \rate_k}{\partial c_m} \qquad
\epsilonPkm       =  \frac{\partial  \rate_k}{\partial p_m}  \nonumber \\
\epsilonSSkmn &=& \frac{\partial^2  \rate_k}{\partial c_m \partial c_n} \qquad
\epsilonSPkmn  =  \frac{\partial^2  \rate_k}{\partial c_m \partial p_n} \qquad
\epsilonPPkmn     =  \frac{\partial^2  \rate_k}{\partial p_m \partial p_n},
\end{eqnarray}
allow us to expand the rate law around a given reference state. The
notion of elasticities can be extended to periodic states.  Sine-wave
oscillations in the metabolite and enzyme levels lead to a periodic state
with oscillating reaction rates.  Shifts and amplitudes of the rate
can be computed, to second order, with the help of periodic
elasticities (see \cite{lieb:2005} and Figure
\ref{fig:periodicelasticities}).  In the model in Box 1, \coout{Figure
\ref{fig:examples}} we considered mass-action kinetics, i.e.~a rate
law that is linear in both $u$ and $x$. Assuming that the enzyme
profiles follow sine functions, we can directly compute the optimal
amplitude and phase (in this case, we obtain a rhythm in phase with
the substrate rhythm).  If a rate law is nonlinear in $x$, computing
the optimal amplitude would be difficult.  However, for small
perturbations, we can expand the rate law around a reference state.  A
rate deviation $\Delta v(t)$, caused by deviations $\Delta u(t)$ and
$\Delta x(t)$, can be approximated by
\begin{eqnarray}
\label{eq:approxrateelasticities}
  \Delta v \approx E_{x} \,\Delta x + E_{u} \,\Delta u + \half E_{xx} \,\Delta x^{2} + E_{ux} \,\Delta u\, \Delta x
\end{eqnarray}
with the unscaled elasticities
$E_{x}=\frac{\partial \rate}{\partial x}$,
$E_{u} = \frac{\partial \rate}{\partial u} = \frac{v}{u}$,
$E_{xx} = \frac{\partial^{2} \rate}{\partial x^{2}}$,
$E_{ux} = \frac{\partial^{2} \rate}{\partial u \partial x} =
\frac{1}{u}\,E_{x}$.
The second-order term $\half\,E_{uu}\, \Delta \eb^2$ does not appear,
since $E_{uu}=0$ (because the enzyme level appears only as a prefactor
in the rate law). To describe oscillations, we consider sine-wave
enzyme profiles $u(t) = \eb + \real(\et\,\e^{i\,\omega\,t})$ and
metabolite profiles $x(t) = \xb + \real(\xt\,\e^{i\,\omega\,t})$ and
determine the flux change caused by $u(t)$, averaged over an
oscillation period $T$. This flux change depends on the last term
only, because the first two terms have vanishing time averages and the
third term does not depend on $u$. Thus, it is only the last term in
Eq.~(\ref{eq:approxrateelasticities}) that matters for periodic enzyme
adaptation. This term resembles the rate law in our mass-action model,
with the mixed elasticity $E_{ux} = \frac{1}{u}\,E_{x}$ replacing the
rate constant $k$.  Enzyme adaptation causes an average rate shift
\begin{eqnarray}
\label{eq:fluxshiftnonlinear}
  \Delta \langle v\rangle_{t} \approx  \real(\half E_{ux} \,\tilde u\, \tilde x)
  = \half   E_{ux} |\tilde u|\, |\tilde x| \cos(\varphi).
\end{eqnarray}
The prefactor
$E_{\tilde u \tilde x} = \half E_{ux} = \frac{E_{x}}{2\,u}$, called
periodic second-order elasticity, translates substrate and enzyme
amplitudes into the resulting flux shifts. For reactions with several
substrates and products, we obtain
\begin{eqnarray}
\label{eq:fluxshiftnonlinearperiodic}
  \Delta \langle v\rangle_{t} \approx \half \real( \et\,\,{\bf E}_{ux} \,\, \tilde \xv),
\end{eqnarray}
where $\tilde \xv$ contains the metabolite amplitudes and
${ \bf E}_{\et \xt} = {\half \bf E}_{ux} = \frac{1}{2u} {\bf E}_{x}$
is the row vector of periodic enzyme-metabolite elasticities. As an
example, consider a reaction $X \leftrightharpoons Y$ with
elasticities $E_{X}>0$ and $E_{Y}\le 0$. With metabolite amplitudes
$\xt$ and $\yt$ a complex enzyme amplitude $\et$, the flux shift reads
$\Delta \langle v \rangle_{t} = \real(\frac{\et}{2\,u}\, (E_{X}\,\xt +
E_{X}\,\yt))$.
For a given amplitude $|\et|$, the flux will be maximal if the enzyme
is in phase with $E_{X}\,\xt + E_{Y}\,\yt$.  In an irreversible
reaction ($E_{Y} = 0$), the optimal enzyme rhythm will be in phase
with X; in reversible reactions, Y will peak after X (phase shift
$0<\varphi<\pi$), and the enzyme will peak before X.

\begin{figure*}[t!]
\parbox{7.5cm}{\includegraphics[width=7.5cm]{\psfilesrhythms/periodic_elasticities.eps}}
\hspace{5mm}
\parbox{7.5cm}{\caption{\small Substrate oscillations lead to periodic
    reaction rates.  The rate law (black curve) translates substrate
    levels (x-axis) into reaction rates (y-axis).  A sine-wave
    substrate oscillation (red curve, where the y-axis symbolises
    time) leads to a non-sine-wave rate oscillation (blue curve, where
    x-axis symbolises time). The minimal and maximal concentrations
    correspond to minimal and maximal rates (dashed lines).  The
    average concentration corresponds to the median rate (dotted
    line), which differs from the average rate (blue straight
    line). In a second-order approximation, the average flux shift can
    be computed from the substrate amplitude by using
    Eq.~(\ref{eq:fluxshiftnonlinear}).  Due to the negative curvature,
    adding a substrate oscillation decreases the average flux. A flux
    increase could be achieved, instead, with a sigmoidal Hill
    kinetics (not shown).}}
\label{fig:periodicelasticities}
\end{figure*}

\subsection{Effective elasticities for periodic metabolic states}
\label{sec:SIperiodicElasticities}

In oscillatory metabolic states, substrate, product, and enzyme levels
vary periodically. To describe how additional (static or periodic)
variations of these profiles will change the (\emph{time-average}
rates or amplitudes of reaction rates, we define \emph{periodic-state
  elasticities}. Using the periodic elasticity matrices (marked by a
circle), the reaction rate profile can be expanded to first order 
(proof in section \ref{sec:SIproofperiodicElasticities})
\begin{eqnarray}
{ \delta \vv \choose    \delta \vvt}
   &=& 
\left(\begin{array}{ll}
  \Eper^{v}_{c}      & \Eper^{v}_{\tilde c}\\
  \Eper^{\tilde v}_{c} & \Eper^{\tilde v}_{\tilde c}\\
\end{array} \right)
{ \delta \cintv \choose    \delta \cintvt}
+
\left(\begin{array}{ll}
  \Eper^{v}_{u}      & \Eper^{v}_{\tilde u}\\
  \Eper^{\tilde v}_{u} & \Eper^{\tilde v}_{\tilde u}\\
\end{array} \right)
{ \delta \uv \choose    \delta \uvt}.
\end{eqnarray}
Close to a static reference state, the effective periodic enzyme
 elasticities are given by 
\begin{eqnarray}
\label{eq:effectivePeriodicEnzymeElasticities}
\left(\begin{array}{ll}
  \Eper^{v}_{u}      & \Eper^{v}_{\tilde u}\\
  \Eper^{\tilde v}_{u} & \Eper^{\tilde v}_{\tilde u}\\
\end{array} \right)
=
\left(\begin{array}{lr}
\diag(\mathring{\vvb})\, \diag(\uvb)\inv & \diag(\mathring{\vvt})\, \diag(\uvb)\inv \\
\diag(\mathring{\vvt})\, \diag(\uvb)\inv &  \diag(\mathring{\vvb})\, \diag(\uvb)\inv
\end{array} \right),
\end{eqnarray}
where $\uvb$ is the average enzyme level, $\mathring{\vvb}=\vv_{\rm
  ref} + \Emat^{\rm v}_{\rm c}\,\Delta \cintvb + \Emat^{\rm v}_{\rm x}\,\Delta \xvb$ is the flux vector in the corresponding average state,
and $\mathring{\vvt} = \Emat^{\rm v}_{\rm c}\, \cintvt +
\Emat^{\rm v}_{\rm x}\,\xvt$.

\subsection{Static and periodic metabolic response coefficients}
\label{sec:ResponseFormulae}

\myparagraph{\ \\Static response coefficients} In a kinetic model with a
given steady reference state, the static and periodic response
coefficients are computed as follows.  With a state vector 
$\ys_{i}(\pv) ={\cvsteady(\pv) \choose \vvsteady(\pv)}$ depending on
system parameters, the static response coefficients
\cite{hesc:96,hohe:93} are defined as
\begin{eqnarray}
  {\RYlpm} &=& \frac{\partial \ys_{l}}{ \partial p_{m}}, \qquad
  {\RYlppsecmatmn} =
  \frac{\partial^{2} \ys_{l}}{ \partial p_{m} \partial p_{n}}.
  \label{eq:RespStationaryDef}
\end{eqnarray}
Using the control matrices \cite{rede:88}
\begin{eqnarray}
 \CSmat =  - \Lmat\, (\NRmat \epsilonSmat \Lmat ) ^{-1} \NRmat, \qquad  \label{eq:CS}
 \CJmat =  \epsilonSmat~ \CSmat + \Imat,   \label{eq:CJ}
\end{eqnarray}
the response matrices can be written as \cite{hohe:93}
\begin{eqnarray}
 \RYpmat &=&  \CYmat ~ \epsilonPmat  \label{eq:RespStationary1} \nonumber \\
 \RYppsecmat &=&  \CYmat\cdot\Gammamat \nonumber \\
\where \Gammamat &=& \epsilonSSmat (\RSmat \otimes \RSmat) 
  +  \epsilonSPmat [\RSmat \otimes \Imat]
  +  \epsilonPSmat [\Imat  \otimes \RSmat] 
  +  \epsilonPPmat. 
\end{eqnarray}

\myparagraph{Spectral response coefficients}  The spectral response
coefficients relate the Fourier components of periodic parameters to
the Fourier components of the responding periodic state variables
\cite{lieb:2005}.  Using the spectral control matrices
\begin{eqnarray}
 \CStmat(\omega) &=&  - \Lmat (\NRmat \epsilonSmat \Lmat - i \omega \Imat) ^{-1} \NRmat  \label{eq:CSsp} \nonumber\\
 \CJtmat(\omega) &=&  \epsilonSmat~ \CStmat(\omega) + \Imat,   \label{eq:CJsp}
\end{eqnarray}
they can be written as
\begin{eqnarray}
 \RspecYpmat(\omega) &=&  \CYtmat(\omega) ~ \epsilonPmat  \label{eq:RespKoeffFirstsp} \nonumber \\
 \RspecYbppsecmat(\omega) &=& \frac{1}{\sqrt{2 \pi}} \CYtmat(0) \cdot\Gammamat(\omega,-\omega) \nonumber \\
 \RspecYtppsecmat(\omega) &=& \frac{1}{\sqrt{2 \pi}} \CYtmat(2 \omega)\cdot\Gammamat(\omega,\omega) \nonumber\\
\where  \Gammamat(\alpha,\beta) &=& 
   \epsilonSSmat [\RspecSpmat(\alpha) \otimes \RspecSpmat(\beta)]
+  \epsilonSPmat [\RspecSpmat(\alpha) \otimes \Imat]
+  \epsilonPSmat [\Imat  \otimes \RspecSpmat(\beta)]
+ \epsilonPPmat. 
\end{eqnarray}
The first-order spectral response coefficients (in the matrix
$\RspecYpmat(\omega)$) relate parameter perturbations to metabolic
effects of the same frequency $\omega$. The second-order spectral
response coefficients (in tensors $\RYbppsecmat(\omega)$ and
$\RYtppsecmat(\omega)$) describe changes of an output variable $z$ at
the frequencies 0 (static shift) and $2 \omega$ (second harmonic).
Details are given in \cite{lieb:2005}. Unfortunatley, there is another
complication.  While spectral response coefficients are defined for
complex Fourier components (i.e.~complex exponentials), the
concentration curves in our models are given by their \emph{real
  parts}: e.g.~$p(t) = \bar p + \real(\e^{i \omega t}\,\pt)$.
Therefore, the coefficients in our formulae are not given by spectral
response coefficients, but by \emph{periodic response coefficients},
which are very similar.  The first-order spectral and periodic
coefficients are completely identical; the second-order periodic
coefficients contain a prefactor $\frac{\sqrt{2 \pi}}{2}$ (see section
\ref{periodicRproof} for a derivation):
\begin{eqnarray}
\label{eq:SpectralAndPeriodic}
 {\RYbppsecmat}(\omega) = \frac{\sqrt{2 \pi}}{2}\, {\RspecYbppsecmat}(\omega), \qquad
 {\RYtppsecmat}(\omega) = \frac{\sqrt{2 \pi}}{2}\, {\RspecYtppsecmat}(\omega).
\end{eqnarray}
For very slow  oscillations (with $\omega \approx 0$), periodic response
 coefficients can be approximated by static response coefficients. The
 second-order coefficients must be divided by 2:
\begin{eqnarray}
  \RYtpmat(\omega\approx0) &\approx&   \RYpmat \nonumber \\
  \RYbppsecmat(\omega\approx0) &\approx&  \half  \RYppsecmat \nonumber \\
  \RYtppsecmat(\omega\approx0) &\approx&  \half  \RYppsecmat.
\end{eqnarray}

\subsection{Periodic mRNA and protein levels}
\label{sec:geneexpression}

Cells can realise protein rhythms by periodic gene expression.
Protein rhythms do not look exactly like their mRNA counterparts, but
are phase-shifted and have smaller relative amplitudes (unless the
amplitudes are increased by ``active'', time-dependent protein
degradation). At high frequencies, protein amplitudes become very
small.  To relate protein rhythms to the underlying mRNA rhythms, we
assume that the protein production rate is proportional to the mRNA
level and that proteins are diluted or linearly degraded (where
regulated protein degradation is not considered).  Under these
assumptions, the protein level $p(t)$ follows the differential
equation
\begin{eqnarray}
\label{eq:proteinProduction}
 \frac{\md p(t)}{\md t} = \alpha\, m(t) - \kappa\, p(t)
\end{eqnarray}
with mRNA concentration $m(t)$, rate constant $\alpha$ for protein
production, and rate constant $\kappa$ for protein degradation
(possibly including enzyme dilution); the values of $\alpha$ and
$\kappa$ may be protein-specific.  With
Eq.~(\ref{eq:proteinProduction}), a sine-wave mRNA profile
$m(t) = \mb + \re(\e^{i \omega t}\,\mt)$ leads to a sine-wave protein
profile $p(t) = \bar p + \re(\e^{i \omega t}\,\tilde p)$ with curve
parameters
\begin{eqnarray}
\bar p &=& \frac{\alpha}{\kappa} \mb, \qquad
\tilde p = \frac{\alpha}{\kappa + i \omega}\, \mt.
\end{eqnarray}
Accordingly,  a desired protein profile $p(t) = \bar p + \re(\e^{i \omega t}\,\tilde
p)$ needs to be realised by an mRNA profile with curve parameters
 \begin{eqnarray} \mb &=&
  \frac{\kappa}{\alpha} \bar p,\qquad \mt = \frac{\kappa + i
    \omega}{\alpha}\, \tilde p.
\end{eqnarray}
To avoid negative mRNA levels, the curve parameters must satify
$\mt \le \mb$. This implies the inequality
$|\tilde p| \le \pt^{\rm max}(\pb,\omega) = (1+\omega/\kappa)^{-1/2}\,
|\bar p|$
for protein amplitudes.  The phase shift between mRNA and protein
peaks is given by $\arctan(\omega/\kappa)$; for very low frequencies
$\omega \approx 0$, mRNA and protein will oscillate in phase; for very
high frequencies, the protein peaks after the mRNA with a phase shift
of $\pi/2$. Proteins with a slow turnover (small $\kappa \gg \omega$)
show weak oscillations and large phase shifts. In contrast, if protein
turnover is fast ($\omega \ll \kappa$), the phase shifts can be
neglected.

\section{Economics of metabolic oscillations}
\label{sec:sioptimaladaption}

To predict optimal enzyme profiles, we need to score such profiles by
a fitness function. Here we consider fitness functions that depend on
external parameters $x_{j}$ and enzyme activities $u_{l}$, and compute
their first and second derivatives.

\subsection{How  static and periodic perturbations affect fitness}

\myparagraph{\ \\Static perturbations shift the metabolic state}
Constant external parameters $x_{j}$ and enzyme activities $u_{l}$
will typically lead to a steady state described by a vector
$\ysv(\xv,\uv) = {\cvsteady(\xv,\uv) \choose \vvsteady(\xv,\uv)}$. If
no such state exists or if it is dynamically unstable, our theory
does not apply. Starting from reference parameters $(\xvref, \uvref)$
and considering static parameter perturbations
${\xv \choose \uv} = {\xvref \choose \uvref} + {\dxvb \choose \duvb}$,
the state variables can be expanded as:
\begin{eqnarray}
\label{eq:fitnessStationary1}
\ysvd &\approx&  (\RYXmat~ \RYUmat) {\dxvb \choose \duvb}
 + \half~
\left( \begin{array}{ll}
\RYsecmat_{\rm xx} & \RYsecmat_{\rm xu}\\
\RYsecmat_{\rm ux} & \RYsecmat_{\rm uu}
 \end{array} \right)
\Big(  {\dxvb \choose \duvb}  \otimes  {\dxvb \choose \duvb} \Big).
\end{eqnarray}
We now consider a fitness function $\ffit = \yy(\ysv(\xv,\uv))
- \hminus(\uv) = \gplus(\xv,\uv) - \hminus(\uv)$.  The {\metabolicobjective} and
cost changes caused by  a parameter change can be expanded to second order:
\begin{eqnarray}
  \label{eq:fitnessStationary2SI}
  \gplus &\approx& \gplus(\uvref) + \qz\cdot \ysvd + \half \ysvd\trans \Qzz \ysvd
   \nonumber\\ 
  \hminus &\approx& \hminus(\uvref) + \hv_{\rm u}\cdot \duvb + \half \duvb\trans \Huu \duvb.
\end{eqnarray}
By inserting the expansions (\ref{eq:fitnessStationary1}) and
(\ref{eq:fitnessStationary2SI}) into our fitness function, we obtain the
perturbed fitness $\ffit(\xvref+\dxvb,\uvref+\duvb)$. Taking derivatives with respect to 
 $\dxvb$ and $\duvb$, we obtain the gradients and the
Hessian matrices (``fitness synergy matrices'')
\begin{eqnarray}
  \label{eq:fitnessStationary3}
  \fv_{\rm \xv}\trans &=& \qz\trans ~\RYXmat \nonumber \\
  \fv_{\rm u}\trans &=& \qz\trans ~\RYUmat -  \hv_{\rm u}\trans\nonumber \\
  \Fux &=& \qz\trans \cdot \RYsecmat_{\rm u\xv} + {\RYUmat}\trans~ \Qzz \RYXmat   \nonumber \\
  \Fuu &=& \qz\trans \cdot \RYsecmat_{\rm u\uv} + {\RYUmat}\trans~ \Qzz \RYUmat - \Huu.
\end{eqnarray}

\myparagraph{Periodic perturbations shift the average metabolic state}
Next, we consider external and enzyme parameters that oscillate around
their reference state (this time, without any shifts of the average values):
\begin{eqnarray}
\xv(t) &=& \xvref+\real(\e^{i \omega t}\,\xvt) \nonumber\\
\uv(t) &=& \uvref+\real(\e^{i \omega t}\,\uvt).
\end{eqnarray}
The time average of $\uv$ is  given by $\uvref$. The average
metabolic state $\ysvb$ can be  expanded  with the help of second-order
periodic response coefficients:
\begin{eqnarray}
\label{eq:fitnessOscillatoryA1SI}
\Delta \ysvb &\approx& \half~
\Big( \begin{array}{ll}
\RYbsecmat_{\rm {\xt\et}} & \RYbsecmat_{\rm {\xt\et}} \\
\RYbsecmat_{\rm {\et\et}} & \RYbsecmat_{\rm {\et\et}}
 \end{array} \Big)
\Big({\xvt \choose \uvt}  \otimes  {\xvt \choose \uvt} \Big).
\end{eqnarray}
There is no first-order term because $\RYbmat_{\rm \xt}$ and
$\RYbmat_{\rm \et}$ vanish (due to time-shift symmetry).  Importantly,
the second-order expansion contains no synergies between static and
periodic perturbation parameters. Therefore, even if both types of
perturbations are present, we can still study them separately by Eqs
(\ref{eq:fitnessStationary1}) and (\ref{eq:fitnessOscillatoryA1SI}).

\subsection{Fitness functionals for periodic metabolic time courses}

\myparagraph{\ \\Fitness functional based on time-averaged state
  variables (``state-average fitness'')}  The fitness
effects of  metabolic rhythms are described  by fitness
functionals, which we obtain from our static fitness function.
As a first possibility, we  apply our  static fitness function
$\ffit = \yy(\ysv(\xv,\uv)) + \hminus(\uv)$ to the time-averaged state
variables (``state-average fitness functional''). Since the time-averaged
enzyme activities remain unchanged ($\duvb=0$), {\metabolicobjective} and cost can
be expanded as
\begin{eqnarray}
  \label{eq:fitnessOscillatoryA2}
  \gplus(\langle \ysv \rangle_{t}) &\approx& \yy(\ysv)
 + \qz\cdot \Delta \ysvb + \half~\Delta \ysvb\trans \Qzz \Delta \ysvb\nonumber \\
  \hminus(\langle \uv \rangle_{t}) &=& \hminus(\uv).
\end{eqnarray}
With Eq.~(\ref{eq:fitnessOscillatoryA1SI}), the derivatives of
$\ffit=\gplus(\langle \ysv \rangle_{t}) - \hminus(\langle \uv
\rangle_{t})$ read
\begin{eqnarray}
  \label{eq:fitnessOscillatoryA3}
  \fv_{\rm \xt}\trans &=& 0 \nonumber \\
  \fv_{\rm \et}\trans &=& 0 \nonumber \\
  \Futxt &=& \qz\trans \cdot \RYbsecmat_{\rm \et \xt} \nonumber \\
  \Futut &=& \qz\trans \cdot \RYbsecmat_{\rm \et \et}.
\end{eqnarray}

\myparagraph{Fitness functional based on time-averaged fitness values
  (``fitness-average fitness'')} As a second  fitness functional
(``fitness-average fitness functional''), the fitness function  is first evaluated in each time
point and then averaged over time. This leads to additional terms in
the  Hessian matrix.  To derive them, we expand the time
courses $\ys(t)$ and the fitness in each time point,
integrate over one oscillation period (duration $T$) and collect all
first- and second-order terms.  For the cost term, we obtain:
\begin{eqnarray}
  \label{eq:fitnessOscillatoryBder1}
  \langle \hminus(\uv) \rangle_{t} &=& \frac{1}{T} \int\limits_{0}^{T} \hminus(\uvref 
   + \real(\e^{i \omega t}\,\uvt ))\, \md t 
 \approx \frac{1}{T} \int\limits_{0}^{T} \hminus(\uvref) 
   + \hv_{\rm u}\cdot \real(\e^{i \omega t}\,\uvt)
   + \half (\e^{i \omega t}\,\uvt)^{\dag} \Huu (\e^{i \omega t}\,\uvt)\,  \md t \nonumber \\
 &=&  \hminus(\uvref) + \frac{1}{4} \uvt^{\dag} \Huu \uvt.
\end{eqnarray}
The first-order term, integrated over time, vanishes. The {\metabolicobjective}
term is computed in a similar way:
\begin{eqnarray}
  \label{eq:fitnessOscillatoryBder2}
 \langle  \gplus(\uv) \rangle_{t} 
 \approx  \gplus(\uv) + \frac{1}{4} \ysvt^{\dag} \Qzz \ysvt 
\quad \where \ysvt = \RYXmat \xvt + \RYUmat \uvt. \nonumber
\end{eqnarray}
Together,  the fitness-average fitness terms
\begin{eqnarray}
  \label{eq:fitnessOscillatoryBder3}
 \langle \gplus(\uv) \rangle_{t}  &\approx& \gplus(\uvref) 
 + \qz\cdot \Delta \ysvb
 + \half \Delta \ysvb\trans \Qzz \Delta \ysvb + \frac{1}{4} \ysvt^{\dag} \Qzz  \ysvt \nonumber \\
\langle  \hminus(\uv) \rangle_{t} &=& \hminus(\uvref) 
+  \frac{1}{4} \uvt^{\dag} \Huu  \uvt
\end{eqnarray}
yield the first and second order derivatives of $\ffit = \langle
\gplus( \ysv) - \hminus(\uv) \rangle_{t} $
\begin{eqnarray}
  \label{eq:fitnessOscillatoryB3}
  \fv_{\rm \xt} &=& 0 \nonumber \\
  \fv_{\rm \et} &=& 0 \nonumber \\
  \Futxt &=& 
   \qz\trans ~\RYbmat_{\rm \et \xt} 
   + \half {\RYtmat_{\rm \et}}^{\dag} \Qzz \RYtmat_{\rm \xt} \nonumber \\
  \Futut &=& \qz\trans ~\RYbmat_{\rm \et \et} 
  + \half {\RYtmat_{\rm \et}}^{\dag} \Qzz \RYtmat_{\rm \et}
  - \half \Huu.
\end{eqnarray}

Since $\RYbppsecmat(\omega=0) = \half \RYppsecmat$, the
frequency-dependent matrices $\Futxt$ and $\Futut$ are given by the
static synergy matrices $\Fux$ and $\Fuu$, divided by a factor of
2. What happens if stationary and periodic perturbations are applied
simultaneously? Since there are no mixed second derivatives,
i.e.~fitness synergies, between stationary and periodic perturbations
(proof in \ref{sec:HigherHarmonics}), the effects of the two
perturbations can  be added.  The derivatives of our fitness
$\Ftemp(\xvref,\uvref;\dxvb,\duvb;\xvt,\uvt)$ with respect to $\dxvb,
\duvb, \xvt$, or $\uvt$ are  given by Eqs   (\ref{eq:fitnessStationary3})
and (\ref{eq:fitnessOscillatoryA3}) or
(\ref{eq:fitnessOscillatoryB3}).

\subsection{Realising a desired metabolic rhythm by  optimal enzyme rhythms}
 \label{sec:achievepredefineddynamic}

 How can we realise a desired metabolic rhythm by a periodic enzyme
 profile?  More precisely, given an external rhythm (with amplitude
 vector $\xvt$), and given desired rhythms of all state variables
 (with amplitude vectors $\cintvt$ and $\vvt$), which enzyme
 amplitudes $\uvt$ will realise these rhythms as closely as possible
 and at a minimal enzyme cost?  The choice of optimal enzyme profiles
 must be self-consistent: each enzyme profile must be adapted to the
 dynamic metabolic state, which arises from the enzyme profiles
 themselves.  Such inverse problems can be hard to solve. However,
 approximations based on {\MCA}, as used in \cite{lksh:04} for steady
 states, make the problems tractable.  To compute the amplitude vector
 $\uvt$, we need to ``invert'' the propagation of oscillations in
 networks. Using a first-order expansion, this is straightforward.
 For sine-wave perturbations of a single frequency, the propagation of
 perturbations in the network can be described by first-order periodic
 response coefficients.  Now we define a goal, for instance, to
 realise a predefined metabolite profile
 $\tilde \cintv \stackrel{!}{=} \Rctut\uvt+\tilde
 R^{\rm \ct}_{\rm \xt}\,\xvt$.
 If the response matrix $\Rctut$ is invertible,
 we can achieve our goal by setting
 $\uvt= {{\Rctut}}$
 $\inv\,[\tilde \cintv - \Rctxt\,\xvt]$. Otherwise, the metabolic behaviour may not be
 precisely realisable, or it may be realisable by more than one enzyme
 profile. In the first case, we employ a least-squares optimisation;
 in the second case, we add a regularisation term to the optimality
 objective (e.g.~a term $\uvt^{\dag}\,\uvt$ favouring small-amplitude
 profiles\footnote{Oscillations of different enzymes could also be
   weighted differently; in models with non-linear investment function
   and fitness-average fitness functional, the cost term
   $\frac{1}{4} \uvt^\dag\,\Huu\,\uvt$ could be used for
   regularisation.}.).  Now the optimality problem for the enzyme
 amplitude vector $\uvt$ reads
\begin{eqnarray} 
\label{eq:optEnzRhythmInverse}
\mbox{Minimise}\quad || (\tilde \cintv - \tilde R^{\cint}_{x}\, \xvt) -
\Rctut \uvt || + \uvt^{\dag}\,\uvt,
\end{eqnarray}
where additional constraints on enzyme or metabolite profiles can be
applied.  Eq.~(\ref{eq:optEnzRhythmInverse}) holds for desired sine-wave
 time profiles $\cintv(t)$.  To realise non-sine-wave time profiles
$\cintv(t)$, we may split the profile into Fourier components, optimise
the enzyme profile for each component, and overlay these profiles by
Fourier synthesis to obtain the enzyme time course $\uv(t)$.  This
procedure, however, may fail in the presence of active enzyme constraints
(e.g.~arising from upper or lower bounds on individual enzyme levels):
if different Fourier modes are coupled by constraints, all these modes
must be optimised simultaneously under constraints.

\subsection{Network-wide enzyme rhythms, described as a series of hypothetical adaptations}
\label{sec:SIiterative}

\myparagraph{\ \\Derivation by considering iterative hypothetical
  adaptations} If we know the periodic fitness synergies between all
model parameters, how can we find a optimal orchestrated enzyme
rhythms? The solution must be self-consistent, i.e.~the enzyme
profiles must be adapted both to external perturbations and to the
metabolic effects of the enzyme profiles themselves.  Such
self-consistent solutions can be approximately found by assuming a
series of hypothetical adaptations.  An oscillating external parameter
will create a direct incentive for enzyme oscillations; for each
enzyme, the optimal amplitude and phase shift are defined by the
complex fitness synergy between enzyme and oscillating parameter.
However, if we realise these enzyme oscillations, their own rhythms
will give rise to new synergy effects between enzyme rhythms, as
described by the elements of $\Futut$. These synergies require
additional adaptations, which create new incentives for further enzyme
adaptation, and so on. By considering the entire series of adaptations
and summing them all up, we obtain exactly the optimal,
self-consistent adaptation predicted by
Eq.~(\ref{eq:optstaticvector}).  We can see this mathematically.  We
first consider an unperturbed, fitness-stable reference state, which
is then perturbed by an external parameter with amplitude $\xt$.  The
elements of $\Fxtut$ describe fitness synergies between the external
parameter and individual enzymes; if enzyme $l$ starts oscillating
with complex amplitude $\et_l$, there will be a synergy term
$\et^*\, F_{\et_l\xt}\,\xt_l$ and a self-synergy term
$\half\,F_{\et_l\et_l}\,\et_l^2$. The self-synergy $F_{\et_l\et_l}$ is
a real number and must be negative (otherwise, there could have been
beneficial self-promoted oscillations of enzyme $l$, which contradicts
our assumption of fitness-stability). The optimal enzyme rhythm -- the
rhythm that maximises the sum of both terms -- reads
\begin{eqnarray}
\et^{(1)}_l &=& - \frac{F_{\et_l\xt}}{F_{\et_l\et_l}}\,\xt.
\end{eqnarray}
This is the direct (or ``first-level'') adaptation.  Now we assume
that all enzymes realise this direct adaptation. For the next
adaptation step, we recalculate the adaptation of our enzyme $l$; with
the existing enzyme rhythms, the {\metabolicobjective} now reads $[\xt\,F_{\xt\et_l}
  + \sum_{j \ne l} \et_j\, F_{\et_j\et_l}] \,\et_l$, and we obtain the
 second-level adaptation
\begin{eqnarray}
  \et^{(2)}_l &=& - \frac{1}{F_{\et_l\et_l}} 
   \left[ F_{\et_l\xt}\,\xt + \sum_{j\ne l} F_{\et_l\et_j}\,\et_j^{(1)} \right]
 = - \frac{1}{F_{\et_l\et_l}} 
   \left[ F_{\et_l\xt}\,\xt - \sum_{j\ne l} F_{\et_l\et_j}\, \frac{F_{\et_j\xt}}{F_{\et_j\et_j}}\,\xt
 \right].
\end{eqnarray}
If we iterate this process, we obtain an infinte series of higher-level
adaptations, and if this series converges, the self-consistent
solution will satify
\begin{eqnarray}
  \et^{(\infty)}_l &=& - \frac{1}{F_{\et_l\et_l}} 
  \left[F_{\et_l\xt}\,\xt + \sum_{j\ne l} F_{\et_l\et_j}\,\et_j^{(\infty)} \right].
\end{eqnarray}
Since $\Futut$ is invertible by assumption, we can solve this equation for the
self-consistent enzyme rhythm:
\begin{eqnarray}
\label{eq:SIseriesExpansionSolution}
\uvt^{(\infty)} &=& - \Futut\inv\, \Futxt\,\xvt.
\end{eqnarray}

\myparagraph{Derivation by expansion of matrix inverse} 
The last step can also be shown differently.  We assume that a
 self-consistent optimal enzyme rhythm exists, and that it is given by
 Eq.~(\ref{eq:SIseriesExpansionSolution}). To break it down into a
 series of adaptation terms, we split our matrix $\Futut$ into a
 matrix $\Amat$ containing the diagonal elements and a matrix $\Bmat$
 containing the off-diagonal elements, and rewrite $\Futut = \Amat
 + \Bmat = \Amat\,[\Imat + \Amat\inv\,\Bmat]$.  Inserting this into
 Eq.~(\ref{eq:SIseriesExpansionSolution}), we obtain
\begin{eqnarray}
\label{eq:SIseriesExpansionSolution2}
\uvt^{(\infty)} &=& - [\Amat\,[\Imat + \Amat\inv\,\Bmat]]\inv\, \Futxt\,\xvt 
\nonumber \\
 &=& - [\Imat + \Amat\inv\,\Bmat]\inv\,\Amat\inv\, \Futxt\,\xvt 
\nonumber \\
 &=& - [\Imat - \Amat\inv\,\Bmat + \Amat\inv\,\Bmat\,\Amat\inv\,\Bmat - ...]\,\Amat\inv\, \Futxt\,\xvt
\nonumber \\
 &=& [- \Amat + \Amat\inv\,\Bmat\,\Amat\inv + \Amat\inv\,\Bmat\,\Amat\inv\,\Bmat\,\Amat\inv - ...]\, \Futxt\,\xvt.
\end{eqnarray}
This is  the same expansion series that we found above.

\subsection{Enzymes that are only promoted by rhythmic states}
\label{sec:RhythmInducedEnzymeActivation}

So far we assumed that all enzymes will be active in our static
reference state. If the enzyme levels are optimal and none of them
hits a bound, the optimality condition tells us that
$\fv_{\rm u} = 0$. What will happen of we abandon this assumption and
consider enzymes that are inactive in the optimal reference state
(that is, hitting the bound at $u_{l}=0$; see Figure
\ref{fig:scenarios} (b))?  If we represent the inactive and active
enzymes by subvectors with subscripts I and A, we obtain the
optimality condition
\begin{eqnarray}
\label{eq:SIrhythminducedStaticGradient}
\fv_{\rm u_{\rm A}}=0, \qquad \fv_{\rm u_{\rm I}} < 0. 
\end{eqnarray}
The situation is illustrated in Figure \ref{fig:scenarios}, with an
active enzyme shown in Figure \ref{fig:scenarios} (a), left; and an
inactive enzyme shown in Figure \ref{fig:scenarios} (b), left.  We can
now expand the fitness function around the reference state like in
Eq.~(\ref{eq:deltafexpansion}).  However, with the non-vanishing
fitness gradient, the expanded fitness function will contain a
first-order term for $\Delta \uv$. \co{HIER kurze erklaerung, was
  jetzt passiert} For generality, we also consider periodically
varying fitness functions, yielding a gradient $\fv_{\rm \et}$ for
enzyme amplitudes $\uvt$. Moreover, instead of referring to an
unperturbed reference state, we allow for an already perturbed
reference state (with external perturbation $\xvt$). The perturbation
will lead to a second-order term
$\real(\xvt^\dag\,\Fxtut\,\uvt)$. Since this term is linear in $\uvt$,
we can include it into the gradient $\fv_{\rm \et}$ and obtain the
effective, complex-valued gradient
$\mathring{\fv}_{\rm \et} = \fv_{\rm \et} + \Futxt\,\xvt$ for enzyme
rhythms.

To predict optimal enzyme profiles, we  expand the fitness
function around  our (static or  perturbed) reference state. 
To first order in $\duvb$ and $\uvt$, and omitting all irrelevant terms, we obtain 
\begin{eqnarray}
\label{eq:boundary1}
  \Delta F(\duvb,\uvt) = \fv_{\rm u} \cdot \duvb 
  + \real([\fv_{\rm \et} + \Futxt\,\xvt] \cdot  \uvt).
\end{eqnarray}
These are the terms that dominate the fitness value close to the
reference state. We now consider our system under external perturbation
$\xvt$, and with a gradient $\fv_{\rm \et}$ representing rhythmic
changes of fitness requirements, and ask whether the enzyme profile
should deviate from its static reference values.  To find an answer,
we maximise Eq.~(\ref{eq:boundary1}) under the constraints
\begin{eqnarray}
\label{eq:boundary1Constraint}
0 \le \uvref + \duvb \le \uv^{\rm max}, \qquad
|\uvt| \le \uvb = \uvref + \duvb
\end{eqnarray}
for static and periodic enzyme variations. We may also consider more
general amplitude constraints $|\uvt| \le \pvt^{\max}(\uvb, \omega)$,
where the vector $|\uvt|$ contains the magnitudes of the elements of
$\uvt$.  The optimality problem can be solved numerically.  To
understand why enzymes stay inactive or why they start oscillating, we
can reformulate the cost function: instead of stating that enzyme
oscillations would imply an increasing average enzyme level (which is
costly), we capture this effect by introducing an effective cost for
enzyme oscillations.  This effective cost concerns only enzymes that
were inactive, and it increases linearly with absolute enzyme
amplitudes (which makes it non-differentiable in the reference state).
To derive a formula for this cost, we reconsider our optimality
problem and assume, as the only constraints, a simple amplitude
constraint for previously inactive enzymes:
$\forall l: u^{\rm ref}_l=0 \Rightarrow |\et|\le \eb_l$.  According to
Eq.~(\ref{eq:SIrhythminducedStaticGradient}), any static change
$\duvb$ would be costly. However, a rhythm in a previously inactive
enzyme \co{GUTES WORT!}  require an increase in their average values:
for matching average values and amplitudes\footnote{The relation
  describes the minimal possible increase in average levels; below
  this, negative enzyme activities would arise. A larger increase, on
  the contrary, would be costly and unnecessary (unless our solution
  hits other constraints, which we excluded here).}, we set $\uvt$ as
$\duvb_{\rm I} = |\uvt|, \duvb_{\rm A} = 0$. By inserting this choice
of $\duvb$ into Eq.~(\ref{eq:boundary1}), we obtain an effective,
amplitude-dependent fitness function
\begin{eqnarray}
\label{eq:SIrhythminducedFexpansion}
 \Ffunctional^{\rm eff}(\uvt) =  \fv_{\rm u}\trans |\uvt|
  + \real([\fv_{\rm \et} + \Futxt \xvt] \cdot \uvt)
\end{eqnarray}
(since $\fv_{\rm u_{\rm I}} = \fv_{\rm u_{\rm I}}$ and
$\fv_{\rm u_{\rm A}} = 0$). The first term is the effective cost of
oscillations, promoted by the amplitude constraint.  What vectors
$\uvt$ will maximise this fitness change?  Given a vector $|\uvt|$, to
maximise the second term, the corresponding elements of $\uvt$ and
$\fv_{\rm \et} + \Futxt \xvt$ must have the same phases, so the
optimal phases of $\uvt$ are given by the phases of
$\fv_{\rm \et} + \Futxt\, \xvt$.  Thus, the effective fitness of an
enzyme rhythm can be written in terms of the real-valued amplitudes
$|\uvt|$:
\begin{eqnarray}
 \Ffunctional^{\rm eff}(\uvt) &=& 
 \fv_{\rm u}\trans |\uvt|  + | \fv_{\rm \et} + \Futxt\, \xvt|\trans \,|\uvt| 
= [\fv_{\rm u}  + |\fv_{\rm \et} + \Futxt\, \xvt|]\trans |\uvt|.
\end{eqnarray}
When optimising $|\uvt|$ with this linear fitness function, the
amplitudes must be bounded. This leads to a constrained linear
programming problem for the real-valued amplitude vector $|\uvt|$. For
example, to study small oscillations (which do not hit any bounds), we
can restrict our amplitude vectors to a small norm
$||\uvt||=\varepsilon$. Maximising the fitness
Eq.~(\ref{eq:SIrhythminducedFexpansion}) under this constraint is
simple: the amplitude vector $\uvt$ is given by the vector
$\fv_{\rm u} + |\fv_{\rm \et} + \Futxt\, \xvt|$, scaled to length
$\varepsilon$.  Thus, in our linear approximation, optimal complex
enzyme amplitudes will given by
$\hat \fv_{\rm u} + |\fv_{\rm \et} + \Futxt\, \xvt|$, multiplied by
some scaling factor. As shown before, the phases of $\uvt$ are given
by the phases of $\fv_{\rm \et} + \Futxt\, \xvt$.

\subsection{Fast enzyme rhythms and the effective cost of posttranslational regulation} 
\label{sec:PosttranslationalCost}

For simplicity, we  assumed so far that the enzyme activities $u_l$ are  given by  enzyme
concentrations, i.e.~protein levels $p_l$. In reality,
enzyme activity can be regulated by posttranslational modification
(e.g.~phosphorylation). This  allows cells to generate fast, strong
enzyme rhythms that cannot achieved by gene expression alone. How
should the two mechanisms be combined to generate  optimal enzyme rhythms? To
describe this, we model the two variables separately: the enzyme
activity $u_l$, representing the concentrations of \emph{active}
enzyme, and the protein level $p_l$ representing the total
concentration of (active plus inactive) enzyme\footnote{For
  simplicity, we assume that an enzyme molecule, depending on
  posttranslational modification states, is either fully active or
  fully inactive; activity is then given by the total enzyme level,
  multiplied by the fraction of active enzymes. In reality, there may
  be multiple modification states with different $k^{\rm cat}$ values,
  which all contribute to the reaction. Our notion of an apparent cost
  still applies in this case. Moreover, there exists also allosteric
  regulation. Here we assume that allosteric regulation is described
  by the rate laws in the metabolic model; however, we could also
  treat it, alternatively, as part of the posttranlational
  modifications.  Finally, fast enzyme oscillations could also be
  achieved transcriptionally by a fast protein turnover, or by
  regulated protein degradation ; however, this may come at an even
  higher cost.}. The fraction of active enzyme molecules (i.e.,
molecules capable of catalysing the reaction) is called
$\rho_{l} = u_l/p_l$.  To realise an enzyme activity $u_l$ (appearing
in the rate laws), a protein level $p_l = u_{l}/\rho_{l}$ (scored by
our enzyme cost function) is needed.  In static enzyme optimisation, a
value of $\rho_l=1$ would be optimal: protein levels and enzyme
activities should be identical, and no posttranslational modifications
is required.  In optimal periodic states, postranslational
modifications may become crucial, because large, fast oscillations
cannot be realised without them. Of course, adding a posttranslational
inhibition will lower the enzyme activities on average, and to
compensate for this effect, the average protein levels must be
increased. This compensation makes the oscillations, effectively,
costly.

We can model this in two ways: we either introduce extra protein variables
$(\pvb, \pvt)$ and couple them to enzyme activities
$(\uvb, \uvt)$ by explicit constraints, or we analyse these
constraints, omit the new variables,  and translate the protein cost $h(\pv)$ into an effective
cost function $h^{\rm eff}(\uvb,\uvt)$ for enzyme activities.  In both
cases, to assign a cost to an enzyme activity profile, we ask how this
profile could be realised at a minimal cost by combining expression
changes and protein modification.  We assume that protein expression
is costly, while protein modification, by itself, comes for free.
Given a desired enzyme activity profile $u(t)$, we search for the
cheapest protein profile $p(t)$ that can realise these enzyme
activities, and consider the cost of this protein profile.  We
consider posttranslational inhibition only (an ``incomplete
activation'' could be treated similarly).  Now I discuss the two
possibilities in more detail.

\myparagraph{1. Explicit constraints} We formulate our optimality problem
in terms of control variables $\uvb, \uvt, \pvb,\pvt, \qv$, and given
perturbation parameters $\xvb$ and $\xvt$. The auxiliary vector $\qv$
is given by $\qv = \max(0,|\uvt| - \pvt^{\rm max})$.  The {\metabolicobjective} and
cost functions $g(\uvb,\uvt,\xvb,\xvt)$ and $h(\pvb,\pvt)$ are
expanded to second order around the reference state. At frequency
$\omega$, we obtain the optimality problem \co{erklaerungen in jeder zeile:}
\begin{eqnarray}
\mbox{Maximize} && g(\uvb,\uvt,\xvb,\xvt) - h(\pvb,\pvt)\quad \mbox{subject to} \nonumber \\
0 &\le& \pvb \le \pvb^{\rm max} \nonumber \\
0 &\le& \uvb \le \pvb \nonumber \\
\qv  &=& \pvb - \uvb  \nonumber \\
|\uvt| &\le& \uvb \nonumber \\
|\pvt| &\le& \pvt^{\rm max}(\pvb,\omega) \nonumber \\
0&\le& |\pvt|  \nonumber \\
|\pvt|  &=& |\uvt| -\qv \nonumber \\
\varphi(\uvt) &=& \varphi(\pvb),
\end{eqnarray}
where $\varphi(\cdot)$ denotes phase angles. The inequalities are
redundant and imply that $\qv\ge 0$.  Close to a static reference
state (which need not be enzyme-optimal), {\metabolicobjective} and cost functions
can be replaced by the quadratic approximation. Writing
$\pvt^{\rm max}(\pvb,\omega) = \gamma(\omega)\,\pvb$ and eliminating
$\pvb$ and $\pvt$, we obtain \co{NOTE: this is what's in the matlab
  scripts!}
\begin{eqnarray}
\mbox{Maximise} && \gu \cdot [\duvb + \qv] + \half\, \real(\uvt^\dag \,\Gutut\,\uvt) + \half\,[\duvb + \qv]\trans \,\Guu\,[\duvb + \qv] + \real(\uvt^\dag \,\Gutxt\,\xvt) \nonumber \\
 \mbox{subject to} &&  \nonumber \\
0 &\le& \uvb   \nonumber \\
\uvb &\le&  \pvb^{\rm max}   \nonumber \\
\qv &\ge&0    \nonumber \\
|\uvt| - \uvb &\le& 0  \nonumber \\
|\uvt| - \qv - \gamma(\omega)\, [\uvb + \qv] &\le& 0\nonumber \\
\qv - |\uvt| &\le& 0\nonumber \\
\uvb + \qv-\pvb^{\rm max} &\le&0
\end{eqnarray}
\co{unklar: nochmal pruefen! was ist mit h? wofuer steht hier delta u
  + q?} 

\myparagraph{2. Effective cost function} Here, \emph{enzyme activities}
$u_l$ are used as the main variables.  An effective cost function
$h(\uvb, \uvt)$, scoring the enzyme activity profiles, is derived from
the given protein cost function $h(\pv)$ (see Figure
\ref{fig:amplitudeConstraint}).  Without posttranslational
modification, enzyme activities $u_l$ and protein levels $p_l$ would
be identical, and for an activity profile $(\uvb,\uvt)$ we would
obtain the following costs and constraints.  With linear costs or
state-average cost functions, the cost is given by a function
$H=h(\uvb) = \sum_l \hul\,\eb_l$. There are two constraints:
$|\et_l| \le \eb_l$, to prevent negative values, and
$|\et_l| \le \pt^{\rm max}_l(\omega,\eb_l)$, representing the maximal
amplitude obtainable from transcription and translation.  In contrast,
with postranscriptional modifications, enzyme activities
$(\uvb, \uvt)$ and protein levels $(\pvb, \pvt)$ can differ. For
optimality reasons, we assume that enzyme activity rhythms are
realised by expression changes whenever possible. If the desired
activity rhythms violate the constraints for protein amplitudes, the
``impossible'' part $q_l=|\et_l|-\pt^{\rm max}_l$ is realised
posttranslationally, by periodic inhibition with amplitude $q_l$ and
in phase with the desired $\et_l$.  Thw inhibition reduces the average
enzyme activity by $q_l$; this must be compensated by increasing the
protein mean value by the same value $q_l$. Thus, to obtain a desired
enzyme amplitude $\et_l$, we set
$q_l = |\et_l|-\pt^{\rm max}_l, |\pt_l| = |\et_l| - q_l$, and
$\pb_l = \eb_l + q_l$. From a linear protein cost function $h(\pv)$,
we obtain the effective cost and constraints

\begin{eqnarray} 
h^{\rm eff}(\uvb,\uvt) = h(\uvb + |\uvt|-\pt^{\rm  max}(\uvb,\omega)), 
\qquad |\et_l| \le \eb_l,\qquad |\et_l| \le \pt_l^{\rm max}(\eb_l + q_l,\omega) + q_l.  
\end{eqnarray}

Formulae for $\pt_l^{\rm max}$, obtained from a simple model of
translation, are given in appendix \ref{sec:computingoptimal} of the
article. They all have the form $\pt_l^{\rm max}(\pb_l,\omega)
= \gamma(\omega)\,\pb_l$, where the prefactor $\gamma(\omega)$
decreases with frequency $\omega$.

\co{NOTE: As mentioned before, instead of explicitly using the effective
  functions and constraints, the $q_l$ can also be introduced as
  additional variables in the quadratic programming problems.}

\section{Example models for metabolic oscillations}
\label{sec:SIexamples}

\subsection{Single reaction with a predefined substrate and product rhythm}
\label{sec:ex1}

Optimal enzyme rhythms in a single reaction are discussed in the
article.  Let us reconsider this calculation with two changes in the
model.  First, I consider a reversible rate law (i.e.~with a rate
affected by substrate and product levels), and second, I use cosine
functions instead of complex exponentials (which is mathematically
equivalent).  I first focus on the dynamics and derive fitness
synergies between metabolite and enzyme rhythms; then I consider optimal
enzyme rhythms, assuming that fitness is given by the average flux
minus a cost that increases quadratically with the enzyme activities.

We consider a single reaction with substrate $X_{1}$ and product
$X_{2}$ (concentrations $x_{1}$ and $x_{2}$). The reaction is
catalysed by an enzyme with activity $u$ and reversible mass-action
kinetics. With all rate constants set to 1 for simplicity, the rate
law reads
\begin{eqnarray}
 v = u (x_{1} - x_{2}).
\end{eqnarray}
The metabolite concentrations are predefined (assuming that our enzyme has no influence 
on metabolite concentrations):
\begin{eqnarray}
  x_{1}(t) &=& \xb_{1} + \xt_{1} \cos(\omega t) \nonumber \\
  x_{2}(t) &=& \xb_{2},
  \label{eq:ex1met1}  
\end{eqnarray}
and we consider enzyme profiles of the form
\begin{eqnarray}
  \u(t) &=& \eb + \et \cos(\omega t + \varphi).
  \label{eq:ex1met1a}  
\end{eqnarray}
To keep $\u$ positive, we require that $\eb \ge 0$ and $|\et| \le
\eb$; the amplitudes $\xt_{1}$ and $\et$ are real numbers and the
phase shift $\varphi$ between $x$ and $u$ can vary between 0 and $2 \pi$.
The time-dependent reaction rate reads 
\begin{eqnarray}
  v(t) &=& (\eb + \et \cos(\omega t + \varphi))( \xb_{1} +
 \xt_{1} \cos(\omega t) - \xb_{2}) \nonumber \\
 &=& \eb \,(\xb_1 -\xb_2)  + \et\, \cos(\omega t + \varphi) (\xb_1 -\xb_2)
 + \eb\, \xt_{1} \cos(\omega t) + \et\, \cos(\omega t + \varphi)
\xt_{1}  \cos(\omega t).
  \label{eq:ex1met1b}  
\end{eqnarray}
The last term describes the synergy between the periodic substrate and
enzyme activities. With the formula $\cos(\alpha)\,\cos(\beta)=
  \half[\cos(\alpha-\beta) + \cos(\alpha+\beta)]$, this term can be rewritten
  as
\begin{eqnarray}
 \et\, \xt_{1} \, \cos(\omega t + \varphi)\, \cos(\omega t) = 
\et\, \xt_{1}  \half\, [\cos(\varphi) + \cos(2 \omega t + \varphi)].
\end{eqnarray}
By averaging the flux (\ref{eq:ex1met1b}) over one oscillation period, we
obtain
\begin{eqnarray}
  \vb &=& \frac{1}{T} \int\limits_{0}^{T} v(t)\, \md t 
  = \eb\, (\xb_1 -\xb_2) + \half \et\, \xt_{1} \cos(\varphi).
  \label{eq:ex1met1c}
\end{eqnarray}
All other terms are periodic and thus average out. The first term in
Eq.~(\ref{eq:ex1met1c}) describes the flux in our steady reference
state; the second term describes a shift caused by the synergy of
metabolite and enzyme rhythms.  In theory, the flux in this model could
be infinitely increased by increasing the enzyme activity. However,
high enzyme activities are costly, and we assume that their cost
increases more than linearly (while the benefit, given by the flux,
increases linearly with the enzyme level)\footnote{To guarantee a
  fitness optimum, {\metabolicobjective} or cost function (or both) must be
  nonlinear. Since we assume a linear {\metabolicobjective} function, a (convex)
  nonlinear investment function is required. If our reaction were part
  of pathway model, the pathway flux (as a {\metabolicobjective} function) would
  typically be a concave, nonlinear function.}. The cost of an enzyme
represents the burden of protein production and maintenance. For
simplicity, we assume that it is given by a positive linear term (a
fixed cost per enzyme molecule) plus a quadratic term (representing an
extra cost if many other enzyme molecules are present).  Thus, the
enzyme cost reads
\begin{eqnarray}
  \hminus(u(t)) &=& \alpha \u(t) + \frac{\beta}{2} \u^{2}(t) \nonumber \\
 &=& \alpha \Big( \eb + \et \cos(\omega t + \varphi) \Big) 
     + \frac{\beta}{2}  \Big( \eb^{2} + 2\, \eb\, \et \cos(\omega t + \varphi) + \et^{2} \cos^{2}(\omega t + \varphi) \Big)
  \label{eq:ex1met1d}  
\end{eqnarray}
with positive coefficients $\alpha$ and $\beta$.
Averaged over time, it becomes
\begin{eqnarray}
 \langle \bar \hminus \rangle_{t} &=& \frac{1}{T} \int\limits_{0}^{T} \hminus(t) \,\md t 
 =  \alpha\, \eb 
     + \frac{\beta}{2}  \eb^{2} + \frac{\beta}{4} \et^{2}
= \hminus(\uvref)  + \frac{\beta}{4} \et^{2}.
  \label{eq:ex1met1e}  
\end{eqnarray}
Like in Eq.~(\ref{eq:ex1met1c}), all single-cosine terms cancel out
and the quadratic cosine term, averaged over an oscillation period,
yields a factor of $\half$.  Compared to the reference state, the cost
increases by $\frac{\beta}{4} \et^{2}$, which depends on the cost
curvature and on the oscillation amplitude.  The fitness function is given by
flux benefit minus enzyme cost, averaged over time:
\begin{eqnarray}
  \Ftemp &=&   \langle y \rangle_{t}- \langle \hminus \rangle_{t}
  = 
  \left( \eb (\xb_1 -\xb_2) + \half \et\, \xt_{1} \cos(\varphi) \right)
  -\left( \alpha \eb 
    + \frac{\beta}{2}   \eb^{2} + \frac{\beta}{4} \et^{2}  \right).
  \label{eq:ex1fit1}
\end{eqnarray}
We now assume a predefined substrate rhythm $\xt_{1}$ with fixed
average metabolite concentration $\xb_{1} > \xb_{2}$ (and a non-oscillating the
product level for simplicity).  To maximise fitness, we choose the
enzyme profile (i.e.~the parameter pair $(\eb, \et)$) that maximises
$\Ftemp$ under the constraints $\eb \ge 0$, $|\et| \le \eb$.  To
optimise $\eb$ and $\et$, we separate the terms that depend on time
averages ($\eb$) from those that depend on oscillations ($\et$ and
$\varphi$):
\begin{eqnarray}
  \Ftemp &=&
 \left(  (\xb_1 -\xb_2 - \alpha) \eb - \frac{\beta}{2} \eb^{2} \right)
+ \left( \half \et \xt_{1} \cos(\varphi) 
     - \frac{\beta}{4}  \et^{2}  \right).
  \label{eq:ex1fit1a}
\end{eqnarray}
Neglecting the inequality constraints for $\eb$ and $\et$, we can
separately maximise the two terms and obtain
\begin{eqnarray}
  \label{eq:ex1locop}
  \eb^{\rm opt} &=&  (\xb_1 -\xb_2 - \alpha)/\beta \nonumber \\
  \cos(\varphi^{\rm opt}) &=& 1 \nonumber \\
  \et^{\rm opt} &=& \xt_1/\beta.
\end{eqnarray}
Setting $\xt=0$, we reobtain the enzyme-optimal reference state
($\et^{\rm opt}=0$). Now we have to check whether our solution
satisfies all constraints.  The solution $\eb^{\rm opt}$ will only be
valid if $\alpha<\xb_{1}-\xb_{2}$: i.e.~already at very small enzyme
activities, the enzyme benefit must exceed the cost; otherwise, a
boundary optimum at $\eb=0$ is obtained (i.e.~the enzyme is not
expressed). Moreover, the optimum for $\et$ holds whenever
$\et^{\rm opt} \le \eb^{\rm opt}$; otherwise, we obtain a boundary
optimum at $\et = \eb^{\rm opt}$.

\iftoggle{bookversion}{}
{
\section{Proofs and derivations}
\label{sec:proofs}

\subsection{Enzyme rhythms can increase fluxes and can evoke second harmonics}
\label{sec:proofFourTerms}

In a single reaction (see Figure \ref{fig:examples} in the main article),
synchronous substrate and enzyme rhythms (represented by quadratic
terms in $\ut$ and $\xt$ in Eq.~(\ref{eq:fluxsplitting})) lead to a
static flux shift (frequency 0) and to a second harmonic (frequency
$2\, \omega$):
\begin{eqnarray}
\real(\ut\,\e^{i\,\omega\,t})\,\real(\xt\,\e^{i\,\omega\,t}) 
&=&
\half (\ut\,\e^{i\,\omega\,t} + \ut^*\,\e^{-i\,\omega\,t})\,
\half (\xt\,\e^{i\,\omega\,t} + \xt^*\,\e^{-i\,\omega\,t}) \nonumber \\
&=&
\frac{1}{4} (\ut\,\xt\, \e^{2\,i\,\omega\,t} + \ut^*\,\xt + \ut\,\xt^* + \ut^*\,\xt^*\,\e^{-2\,i\,\omega\,t}) \nonumber \\
&=&
\half \real(\ut\,\xt\, \e^{2\,i\,\omega\,t}) + \half\, \real(\ut^*\,\xt).
\end{eqnarray}

\subsection{Effective elasticities in periodic metabolic states}
\label{sec:SIproofperiodicElasticities}

In periodic metabolic states, the changes of average fluxes and flux
amplitudes caused by small (static or periodic) perturbations can be
described by effective reaction elasticities.  To derive formula
(\ref{eq:effectivePeriodicEnzymeElasticities}), we first consider a
static reference state with internal metabolite concentrations
$\cv_{\rm ref}$, external metabolite concentrations $\xv_{\rm ref}$, and
enzyme levels $\uv_{\rm ref}$.  Close to this state, the
time-dependent reaction rates can be expanded as
\begin{eqnarray}
\label{eq:oscVExpansion}
  \vv(t) &\approx& \vv_{\rm ref} + 
  \left(\begin{array}{r} 
    \Emat^{\rm v}_{\rm c} \\ \Emat^{\rm v}_{\rm x} \\  \Emat^{\rm v}_{\rm u}  
  \end{array}\right)\trans
  \left(\begin{array}{r} 
    \Delta \cv(t)\\ \Delta \xv(t) \\ \Delta \uv(t)
  \end{array}\right) \nonumber \\
 && + \half
 \left(\begin{array}{r} \Delta \cv(t)\\ \Delta \xv(t) \\ \Delta \uv(t)  
\end{array}\right)\trans
   \left(\begin{array}{rrr} 
     \Emat^{\rm v}_{\rm cc} & \Emat^{\rm v}_{\rm cx} &  \Emat^{\rm v}_{\rm cu}\\
     \Emat^{\rm v}_{\rm xc} & \Emat^{\rm v}_{\rm xx} &  \Emat^{\rm v}_{\rm xu}\\
     \Emat^{\rm v}_{\rm uc} & \Emat^{\rm v}_{\rm ux} &  \Emat^{\rm v}_{\rm uu}
\end{array}
\right)
\left(\begin{array}{r} \Delta \cv(t)\\ \Delta \xv(t) \\ \Delta \uv(t)
\end{array}\right)
\end{eqnarray}
with a reference {\flow}
$\vv_{\rm ref} = \nonumber \vv(\cv_{\rm ref},\xv_{\rm ref},\uv_{\rm
  ref})$, and
\begin{eqnarray}
 \cv(t) &=& \cv_{\rm ref} + \Delta \cv(t) \nonumber \\
 \xv(t) &=& \xv_{\rm ref} + \Delta \xv(t) \nonumber \\
 \uv(t) &=& \uv_{\rm ref} + \Delta \uv(t).
\end{eqnarray}
We now consider a state with periodic metabolite and enzyme
profiles
\begin{eqnarray}
\label{eq:PerElasticityProfiles}
 \cv(t) &=& \cv_{\rm ref} + \Delta \cvb + \real(\cvt\,\e^{i \omega t}) \nonumber \\
 \xv(t) &=& \xv_{\rm ref} + \Delta \xvb + \real(\xvt\,\e^{i \omega t}) \nonumber \\
 \uv(t) &=& \uv_{\rm ref} + \Delta \uvb + \real(\uvt\,\e^{i \omega t}).
\end{eqnarray}
In a first-order expansion, the reaction rates show a sine-wave
time dependence
\begin{eqnarray}
 \vv(t) &\approx& \vv_{\rm ref} + \Delta \vvb + \real(\vvt\,\e^{i \omega t}).
\end{eqnarray}
By equating this to  Eq.~(\ref{eq:oscVExpansion}), with
the profiles (\ref{eq:PerElasticityProfiles}) inserted, we obtain equations for the
expansion terms
\begin{eqnarray}
\label{eq:PerElasticityVExpansion}
  \Delta \vvb  &=& 
  \left(\begin{array}{r} 
    \Emat^{\rm v}_{\rm c} \\ \Emat^{\rm v}_{\rm x} \\  \Emat^{\rm v}_{\rm u}  
  \end{array}\right)\trans
  \left(\begin{array}{r} 
    \Delta \cvb\\ \Delta \xvb \\ \Delta \uvb
  \end{array}\right)
+ \half 
 \left(\begin{array}{r} \Delta \cvb\\ \Delta \xvb \\ \Delta \uvb  
\end{array}\right)\trans
   \left(\begin{array}{rrr} 
     \Emat^{\rm v}_{\rm cc} & \Emat^{\rm v}_{\rm cx} &  \Emat^{\rm v}_{\rm cu}\\
     \Emat^{\rm v}_{\rm xc} & \Emat^{\rm v}_{\rm xx} &  \Emat^{\rm v}_{\rm xu}\\
     \Emat^{\rm v}_{\rm uc} & \Emat^{\rm v}_{\rm ux} &  \Emat^{\rm v}_{\rm uu}
\end{array}
\right)
\left(\begin{array}{r} \Delta \cvb\\ \Delta \xvb \\ \Delta \uvb
\end{array}\right) \nonumber \\
&&+ \half
 \left(\begin{array}{r}  \cvt\\  \xvt \\  \uvt  
\end{array}\right)^\dag
   \left(\begin{array}{rrr} 
     \Emat^{\rm v}_{\rm cc} & \Emat^{\rm v}_{\rm cx} &  \Emat^{\rm v}_{\rm cu}\\
     \Emat^{\rm v}_{\rm xc} & \Emat^{\rm v}_{\rm xx} &  \Emat^{\rm v}_{\rm xu}\\
     \Emat^{\rm v}_{\rm uc} & \Emat^{\rm v}_{\rm ux} &  \Emat^{\rm v}_{\rm uu}
\end{array}
\right)
\left(\begin{array}{r}  \cvt\\  \xvt \\  \uvt
\end{array}\right)
 \nonumber \\
\vvt &=& 
  \left(\begin{array}{r} 
    \Emat^{\rm v}_{\rm c} \\ \Emat^{\rm v}_{\rm x} \\  \Emat^{\rm v}_{\rm u}  
  \end{array}\right)\trans
  \left(\begin{array}{r} 
     \cvt\\  \xvt \\  \uvt
  \end{array}\right)
+  \left(\begin{array}{r} \Delta \cvb\\ \Delta \xvb \\ \Delta \uvb  
\end{array}\right)\trans
   \left(\begin{array}{rrr} 
     \Emat^{\rm v}_{\rm cc} & \Emat^{\rm v}_{\rm cx} &  \Emat^{\rm v}_{\rm cu}\\
     \Emat^{\rm v}_{\rm xc} & \Emat^{\rm v}_{\rm xx} &  \Emat^{\rm v}_{\rm xu}\\
     \Emat^{\rm v}_{\rm uc} & \Emat^{\rm v}_{\rm ux} &  \Emat^{\rm v}_{\rm uu}
\end{array}
\right)
\left(\begin{array}{r}  \cvt\\  \xvt \\ \uvt
\end{array}\right).
\end{eqnarray}
We now consider our  periodic state (defined by a steady reference state
and additional changes $\Delta \cv, \Delta \xv, \Delta \uv$, and 
$\cvt, \xvt, \uvt$) and study the effects of small additional enzyme
variations (defined by $\delta \uv$ and $\delta \uvt$). We expand the flux
variation to first order
\begin{eqnarray}
\label{eq:PerElasticityVExpansionX}
{ \delta \vv \choose    \delta \vvt}
   &=& 
\left(\begin{array}{ll}
  \Eper^{v}_{u}      & \Eper^{v}_{\tilde u}\\
  \Eper^{\tilde v}_{u} & \Eper^{\tilde v}_{\tilde u}\\
\end{array} \right)
{ \delta \uv \choose    \delta \uvt},
\end{eqnarray}
with expansion coefficients in the matrix still to be determined.
Using Eq.~(\ref{eq:PerElasticityVExpansion}), and noting that
$\Emat^{\rm v}_{\rm uu}=0$, we  obtain the expansion
\begin{eqnarray}
\delta \vv   &=& 
 [\Emat^{\rm v}_{\rm u} + \Delta \cvb\trans \Emat^{\rm v}_{\rm cu} 
  + \Delta \xvb\trans \Emat^{\rm v}_{\rm xu}]\, \delta \uvb 
 +  [\cvt^\dag \Emat^{\rm v}_{\rm cu}  + \xvt^\dag \Emat^{\rm v}_{\rm xu}]\,\delta \uvt
 \nonumber \\
 \delta \vvt   &=& 
   [\cvt^\dag \Emat^{\rm v}_{\rm cu}  + \xvt^\dag \Emat^{\rm v}_{\rm xu}]\,\delta \uvb 
 + [\Emat^{\rm v}_{\rm u} +  \Delta \cvb\trans \Emat^{\rm v}_{\rm cu} 
    + \Delta \xvb\trans \Emat^{\rm v}_{\rm xu}]\,\delta \uvt.
\end{eqnarray}
By comparing this to Eq.~(\ref{eq:PerElasticityVExpansionX}), 
we obtain the effective elasticities 
\begin{eqnarray}
  \Eper^{v}_{u}  &=&   \Eper^{\tilde v}_{\tilde u} =  \Emat^{\rm v}_{\rm u} + \Delta \cvb\trans \Emat^{\rm v}_{\rm cu}  + \Delta \xvb\trans \Emat^{\rm v}_{\rm xu} \nonumber \\
  \Eper^{v}_{\tilde u} &=&    \Eper^{\tilde v}_{u} = 
 \cvt^\dag \Emat^{\rm v}_{\rm cu}  + \xvt^\dag \Emat^{\rm v}_{\rm xu}.
\end{eqnarray}
Since the  enzyme levels are prefactors in the rate laws, we
can set $\Emat^{\rm v_l}_{\rm u_l} = \frac{v_l}{u_l}$, $\Emat^{\rm
  v_l}_{\rm c_i u_l} = \Emat^{\rm v_l}_{\rm c_i} / u_l$, $\Emat^{\rm
  v_l}_{\rm x_i u_l} = \Emat^{\rm v_l}_{\rm x_i}/u_l$, and $\Emat^{\rm
  v}_{\rm uu} = 0$ and thus rewrite the effective elasticities as 
\begin{eqnarray}
  \Eper^{v}_{u}  &=&   \Eper^{\tilde v}_{\tilde u} = \diag(\uvb)\inv\,
  \diag(\vv_{\rm ref} + \Emat^v_c\,\Delta \cvb + \Emat^v_x\,\Delta \xvb)
  = \diag(\uvb)\inv\,\diag(\mathring{\vvb}) \nonumber \\
  \Eper^{v}_{\tilde u} &=&    \Eper^{\tilde v}_{u} = \diag(\uvb)\inv\,
  \diag(\Emat^v_c\,\Delta \cvt + \Emat^v_x\,\Delta \xvt) 
  = \diag(\uvb)\inv\,\diag(\mathring{\vvt}),
\end{eqnarray}
where we defined $\mathring{\vvb} = \vv_{\rm ref} + \Emat^{\rm v}_{\rm c}\,\Delta
\cvb + \Emat^{\rm v}_{\rm x}\,\Delta \xvb$ 
and $\mathring{\vvt} = \Emat^{\rm
  v}_{\rm c}\, \cvt + \Emat^{\rm v}_{\rm x}\,\xvt$. Altogether, we
obtain the elasticity matrices
\begin{eqnarray}
\label{eq:effectivePeriodicEnzymeElasticitiesProof}
\left(\begin{array}{ll}
  \Eper^{v}_{u}      & \Eper^{v}_{\tilde u}\\
  \Eper^{\tilde v}_{u} & \Eper^{\tilde v}_{\tilde u}\\
\end{array} \right)
=
\left(\begin{array}{lr}
\diag(\mathring{\vvb})\, \diag(\uvb)\inv & \diag(\mathring{\vvt})\, \diag(\uvb)\inv \\
\diag(\mathring{\vvt})\, \diag(\uvb)\inv &  \diag(\mathring{\vvb})\, \diag(\uvb)\inv
\end{array} \right).
\end{eqnarray}
Effective periodic elasticities with respect to reactant
levels $\cv$ or $\xv$ can be derived in a similar way.

\co{DON'T need to write: All other expansion terms vanish because (i) the second-order
  enzyme elasticities $\Emat^{v}_{uu}$ vanish; (ii) metabolite
  variations vanish; and (iii) terms between perturbations of
  different frequencies vanish (e.g.~the coupling of two static
  variations cannot yield a periodic variation).  Note that the symbol
  $\real(\cdot)$ is omitted in the following, and real parts must be
  taken whenever real numbers are required (e.g.~for average shifts,
  or for fitness changes).}

\subsection{Periodic response coefficients Eq.~(\ref{eq:SpectralAndPeriodic})}
\label{periodicRproof}

\co{REMOVE?  The usage of periodic response coefficients, instead
  of the spectral response coefficients defined before, is a matter of
  convenience. A real-valued cosine oscillation can be written as a
  sum $\cos(\omega\,t) =
  \half\,[u\,\e^{i\,\omega\,t}+u^*\,\e^{-i\,\omega\,t}]$, i.e.~it is
  a sum of complex-valued oscillations of frequency $\omega$ and
  $-\omega$.  Spectral response coefficients refer to these individual
  complex-valued oscillations.  The expansion formulae in our
  formalism, however, refer only the do not consider this
  splitting. In the second-order expansion, }

Periodic and spectral response coefficients differ by a prefactor,
which we will now derive. For Fourier transformations, we adopt the
prefactor convention from \cite{lieb:2005}
\begin{eqnarray}
  x(t) = \frac{1}{\sqrt{2 \pi}} \int \xt \,\e^{i\,\omega\,t} \md t, \qquad
  \xt(\omega) = \frac{1}{\sqrt{2 \pi}} \int  x \,\e^{-i\,\omega\,t} \md t.
\end{eqnarray}
A real-valued, sine-wave parameter perturbation
\begin{eqnarray}
 \pvd(t) &=& \real[\pvt\, \e^{i \omega t}]
 = \half \left[\pvt\, \e^{i \omega t} + \pvt^{*}\, \e^{-i \omega t} \right],
\end{eqnarray}
with  complex amplitude vector $\pvt$, has the Fourier
transform
\begin{eqnarray}
\hat{\pv}(\alpha) = \frac{\sqrt{2 \pi}}{2} \, \delta_{\alpha}(\omega)~\pvt  + 
\frac{\sqrt{2 \pi}}{2} \, \delta_{\alpha}(-\omega)~\pvt^{*}.
\end{eqnarray}
The Fourier components of a state variable $\ys$ can be approximated
with the help of spectral response cofficients $\RspecYpmat$, the
functional derivatives between Fourier components \cite{lieb:2005}.
In a first-order expansion, the Fourier components of $\ys$, at
frequency $\alpha$, read
\begin{eqnarray}
\label{eq:fourierfirstorder}
\hat{\ysv}(\alpha) &\approx&   \RspecYtpmat(\alpha)~ \hat{\pv}(\alpha) 
=  
\frac{\sqrt{2 \pi}}{2} ~\,\delta_{\alpha}(\omega)~ \RspecYtpmat(\omega)~   \pvt 
 + \frac{\sqrt{2 \pi}}{2}\,\delta_{\alpha}(-\omega) ~\RspecYtpmat(-\omega)~\pvt^{*}.
\end{eqnarray}
By applying a reverse Fourier transformation, we obtain the
temporal behaviour
\begin{eqnarray}
\ysvd(t) &\approx& 
  \frac{1}{2} ~ 
 \left( \RspecYtpmat(\omega)~\pvt~\e^{i \omega t} + \RspecYtpmat(-\omega)\, \pvt^{*} \e^{-i \omega t} \right) = 
\real[ \RspecYtpmat(\omega)\, \pvt\, \e^{i \omega t}],
\end{eqnarray}
where we used the fact that $\RspecYtpmat(-\omega)$ and
$\RspecYtpmat(\omega)$ are complex conjugates.  Thus, the
periodic response coefficient, defined as the first-order expansion cofficient
appearing in this formula, is given by the spectral
response cofficient $\RspecYtpmat(\omega)$.  Now we consider a
second-order expansion.  An expansion with spectral response
cofficients yields additional terms in the Fourier transform, which
need to be added to Eq.~(\ref{eq:fourierfirstorder}):
\begin{eqnarray}
&&  \delta_{\alpha}(0)\,  \RspecYbppsecmat(\omega)  \left(\frac{\sqrt{2 \pi}}{2}  \pvt \otimes \frac{\sqrt{2 \pi}}{2} \pvt^{*} \right) \nonumber \\
&&+ \frac{1}{2}\, \delta_{\alpha}(2 \omega) \RspecYtppsecmat(\omega) \left(\frac{\sqrt{2 \pi}}{2}  
 \pvt \otimes \frac{\sqrt{2 \pi}}{2} \pvt \right)
 + \frac{1}{2}\,\delta_{\alpha}(-2 \omega)
 \RspecYtppsecmatconj(\omega) \left(\frac{\sqrt{2 \pi}}{2} \pvt^{*} \otimes \frac{\sqrt{2 \pi}}{2}\pvt^{*} \right) \nonumber \\
&=& \frac{ 2 \pi}{4} \left(
  \delta_{\alpha}(0)\,  \RspecYbppsecmat(\omega)  \left[ \pvt \otimes \pvt^{*} \right]
+ \frac{1}{2}\, \delta_{\alpha}(2 \omega)\, \RspecYtppsecmat(\omega) \left[
 \pvt \otimes  \pvt \right]
 + \frac{1}{2}\,\delta_{\alpha}(-2 \omega)\,
 \RspecYtppsecmatconj(\omega) \left[ \pvt^{*} \otimes \pvt^{*} \right] \right)
\end{eqnarray}
In the time domain (Eq.~(\ref{eq:fitnessOscillatoryA2})), we obtain
the additional terms
\begin{eqnarray}
 && ... + \frac{\sqrt{2 \pi}}{4} \left(
   \RspecYbppsecmat(\omega) [\pvt \otimes  \pvt^{*}]
  + \frac{1}{2}\RspecYtppsecmat(\omega) [\pvt \otimes \pvt]\, \e^{i 2 \omega t}
   +    \frac{1}{2} \RspecYtppsecmatconj(\omega) [\pvt^{*} \otimes  \pvt^{*}]
  \e^{-2 i \omega t}
\right) \nonumber \\
 &=&... 
   + \frac{1}{2} \real \left(\frac{\sqrt{2 \pi}}{2} \RspecYbppsecmat(\omega) 
[ \pvt \otimes \pvt^{*} ] \right)
   + \frac{1}{2} \real \left(\frac{\sqrt{2 \pi}}{2}\RspecYtppsecmat(\omega) [\pvt \otimes  \pvt]  \e^{2 i \omega t} \right).
\end{eqnarray}
The periodic response coefficients (i.e.~the expansion coefficients
in this formula) read
\begin{eqnarray}
 {\RYbppsecmat}(\omega) = \frac{\sqrt{2 \pi}}{2}\, {\RspecYbppsecmat}(\omega), \qquad
 {\RYtppsecmat}(\omega) = \frac{\sqrt{2 \pi}}{2}\, {\RspecYtppsecmat}(\omega).
\end{eqnarray}
Again, they are given by the spectral response coefficients, but now
with a prefactor $\frac{\sqrt{2\,\pi}}{2}$.

\subsection{There are no  fitness synergies between higher harmonics}
\label{sec:HigherHarmonics}

\co{does this result depend on our second-order expansion? mention this clearly!}

Why can rhythms of different frequencies be treated separately?  In
our fitness expansion Eq.~(\ref{eq:deltafexpansion}), fitness
contributions at different frequencies appear independently;
therefore, higher harmonics of enzyme rhythms can be optimised
separately, unless they are coupled by constraints.  This will be
shown now.  For a simple notation, we merge all rhythmic parameters in
a vector $\pv = {\xv \choose \uv}$. Our fitness functional
$\Ffunctional$ depends on time-average values (e.g.~average benefit
$\langle b\rangle_t$, average cost $\langle h\rangle_t$, average
concentrations and fluxes $\langle \cv \rangle_t$ and
$\langle \vv\rangle_t$). We assume that the functional is invariant
against time shifts, so a shifted profile $\pv(t+\Delta t)$ will yield
the same fitness value as $\pv(t)$.  After expanding $\pv(t)$ into a
Fourier series
$\pv(t) = \pv_{(0)} + \pvt_{(\omega)}\,\e^{i\,\omega\,t} +
\pvt_{(2\omega)}\,\e^{i\,\omega\,t} + ..$,
we can write the functional as a function
$f(\pv_{(0)}, \pvt_{(\omega)}, \pvt_{(2\omega)}, ..)$.  Now we expand
$f$ into a power series around a reference state $\pv_{\rm ref}$:
\begin{eqnarray}
\label{eq:fitnessTaylorExpansion}
f &=& f(\pv_{\rm ref}) + f_\pv \cdot \Delta \pvb
+ f_{\pv,\omega} \cdot \pvt_{(\omega)}
+ f_{\pv,2\omega} \cdot  \pvt_{(2\omega)} + ... \nonumber \\
&&+ \half
\left(\begin{array}{l}
\Delta \pvb \\  \pvt_{(\omega)}\\ \pvt_{(2\omega)}\\.. 
\end{array}\right)^\dag
\left(\begin{array}{llll}
\Fmat_{\pvb \pvb} & \Fmat_{\pvb \pvt_{(\omega)}} & \Fmat_{\pvb \pvt_{(2\omega)}} & .. \\
\Fmat_{\pvt_{(\omega)} \pvb} & \Fmat_{\pvt_{(\omega)} \pvt_{(\omega)}} & \Fmat_{\pvt_{(\omega)} \pvt_{(2\omega)}} & .. \\
\Fmat_{\pvt_{(2\omega)} \pvb  } & \Fmat_{\pvt_{(2\omega)} \pvt_{(\omega)}} & \Fmat_{\pvt_{(2\omega)} \pvt_{(2\omega)}} & .. \\
..&..&..&..
\end{array}\right)
\left(\begin{array}{l}
\Delta \pvb \\  \pvt_{(\omega)}\\ \pvt_{(2\omega)}\\.. 
\end{array}\right),
\end{eqnarray}
where $\pv(0) = \pv_{\rm ref} + \Delta \pvb$.
Time-shift invariance, $\Ffunctional[\pv(t)] = {\mathcal
  F}[\pv(t+\Delta t)]$, yields the condition
\begin{eqnarray}
f(\pv_{(0)}, \pvt_{(\omega)}, \pvt_{(2\omega)}, ..)
= f(\pv_{(0)}, \pvt_{(\omega)}\,\e^{i\,\omega\,\delta t}, 
             \pvt_{(2\omega)}\,\e^{2 i\,\omega\,\delta t}, ..).
\end{eqnarray}
Thus, in order to satisfy time-shift invariance,
Eq.~(\ref{eq:fitnessTaylorExpansion}) must yield the same result if we
replace
$\pvt_{(\omega)} \rightarrow \pvt_{(\omega)}\,\e^{i\,\omega\,\delta
  t}$,
$ \pvt_{(2\omega)} \rightarrow \pvt_{(2\omega)}\,\e^{2
  i\,\omega\,\delta t}$,
and so on, for any choice of $\delta t$. In order for this to hold,
all linear terms for periodic parameters (i.e, $f_{\pv,\omega}$,
$f_{\pv,2\omega}$, ..) must vanish, and all mixed quadratic terms for
different frequencies (e.g.~$\Fmat_{\pvt_{(\omega)} \pvb}$) must
vanish as well. For the non-mixed quadratic terms
(e.g.~$\Fmat_{\pvt_{(\omega)}\pvt_{(\omega)}}$), invariance holds
because the factor $\e^{i\,\omega\,\delta t}$ appears on both sides
(once as a complex conjugate) and thus cancels out. We obtain an
expansion of the form
\begin{eqnarray}
f &=& f(\pv_{\rm ref}) + \half
\left(\begin{array}{l}
\Delta \pvb \\  \pvt_{(\omega)}\\ \pvt_{(2\omega)}\\.. 
\end{array}\right)^\dag
\left(\begin{array}{llll}
\Fmat_{\pvb \pvb} & 0 & 0 & .. \\
0 & \Fmat_{\pvt_{(\omega)} \pvt_{(\omega)}} & 0 & .. \\
0 & 0 & \Fmat_{\pvt_{(2\omega)} \pvt_{(2\omega)}} & .. \\
..&..&..&..
\end{array}\right)
\left(\begin{array}{l}
\Delta \pvb \\  \pvt_{(\omega)}\\ \pvt_{(2\omega)}\\.. 
\end{array}\right) \nonumber \\
 &=& f(\pv_{\rm ref})
+ \half  \Delta \pvb^\dag\,\Fmat_{\pvb \pvb}\,\Delta \pvb
+ \half \pvt_{(\omega)}^\dag\,  \Fmat_{\pvt_{(\omega)} \pvt_{(\omega)}}\, \pvt_{(\omega)}
+ \half \pvt_{(2\omega)}^\dag \,  \Fmat_{\pvt_{(2\omega)} \pvt_{(2\omega)}} \,  \pvt_{(2\omega)}
+ ...
\end{eqnarray}
Since the parameter vector $\pv$ comprises both $\xv$ and $\uv$, each
quadratic term can be split into separate terms for
external-external, external-enzyme, and enzyme-enzyme synergies.

\subsection{Optimal enzyme rhythms under constraints, Eq.~(\ref{eq:SolutionWithConstraints})}
\label{sec:RhythmConstraintsLagrange}

To derive optimal enzyme profiles under constraints,
Eq.~(\ref{eq:SolutionWithConstraints}), we consider the quadratic
optimality problem (\ref{eq:OptimalityProblem}).  As constraints, we
consider bounds for the central values $0 \le \uvb \le \uvb^{\rm max}$
as well as amplitude constraints (either simple positivity constraints
$|\uvt| \le \uvb$ or frequency-dependent constraints based on protein
production, $|\uvt| \le \pvt^{\rm max}(\uvb,\omega)$).  The fitness
function for control variables ($\duvb$, and $\uvt$) and external
variables ($\dxvb$, $\xvt$) reads
\begin{eqnarray}
\label{eq:ExpansionSIA1}
F = \duvb\trans \,\Fux \,\dxvb + 
\half \duvb\trans\,\Fuu\,\duvb +
\real(\uvt^\dag\, \Futxt \,\xvt) + \half\,\uvt^\dag\, \Futut \,\uvt,
\end{eqnarray}
where constant terms have been omitted.  The constraints $0 \le \uvb$,
$\uvb \le \uvb^{\rm max}$, and $|\uvt| \le \pvt^{\rm
  max}(\uvb,\omega)$ can be described by defining
\begin{eqnarray}
 a &=& -\uvb \nonumber \\
 b &=&  \uvb - \uvb^{\rm max} \nonumber \\
 c &=& |\uvt| - \pvt^{\rm max}(\uvb,\omega).
\end{eqnarray}
and requiring $a\le 0, b\le 0, c\le0$.
Using real-valued Lagrange multiplier vectors $\alphav$, $\betav$,
and $\gammav$, we can reformulate the optimality problem 
and obtain the Kuhn-Tucker optimality conditions
\begin{eqnarray}
\label{eq:ExpansionKuhnSIA2}
0 &=& \frac{\partial F}{\partial \duvb} +
   \alphav \cdot\frac{\partial a}{\partial \duvb} 
 + \betav  \cdot\frac{\partial b}{\partial \duvb} 
 + \gammav \cdot\frac{\partial c}{\partial \duvb}  \nonumber \\
0 &=& \frac{\partial F}{\partial \uvt} +
   \alphav \cdot\frac{\partial a}{\partial \uvt} 
 + \betav  \cdot\frac{\partial b}{\partial \uvt} 
 + \gammav \cdot\frac{\partial c}{\partial \uvt},
\end{eqnarray}
where all Lagrange multipliers must be  positive (or zero, if the
corresponding constraint is not active). After inserting
Eq.~(\ref{eq:ExpansionSIA1}), we can rewrite
Eq.~(\ref{eq:ExpansionKuhnSIA2}) as
\begin{eqnarray}
\Fux \,\dxvb + \Fuu\,\duvb &=& -\alphav + \betav 
 - \gammav \cdot\frac{\partial \pvt^{\rm max}(\uvb,\omega)}{\partial \duvb}
  \nonumber \\
\Futxt \,\xvt +  \Futut \,\uvt &=& 
\gammav \cdot \frac{\partial |\uvt|}{\partial \uvt}.
\end{eqnarray}
Noting that  $\frac{\partial \pvt^{\rm max}(\uvb,\omega)}{\partial \duvb} =
\diag(\pvt^{\rm max}/\duvb) = \diag(\pvt^{\rm max}_{\rm rel}(\omega))$
and $\frac{\partial |\uvt|}{\partial \uvt} = \diag(\uvt/
|\uvt|)$, and merging $-\alphav$ and $\betav$ into a vector $\muv$, we
 obtain
\begin{eqnarray}
\label{eq:ExpansionKuhnSIA3}
\Fux \,\dxvb + \Fuu\,\duvb &=& \muv
 - \diag(\pvt^{\rm max}_{\rm rel}(\omega))\, \gammav \nonumber \\
\Futxt \,\xvt +  \Futut \,\uvt &=& \diag\left(\frac{\uvt}{|\uvt|}\right)\, \gammav,
\end{eqnarray}
where $\mu_l<0$ for inactive enzymes (i.e.~$\ub_l=0$), $\mu_l>0$ for
 enzymes whose central value $\ub_l$ hits the upper bound, and
$\mu_l=0$ otherwise. Similarly, $\gamma_l>0$ holds for all enzymes with active
amplitude constraints, and $\gamma_l=0$ otherwise.  
Eq.~(\ref{eq:ExpansionKuhnSIA3}) can be solved for the 
optimal enzyme profiles
\begin{eqnarray}
\duvb &=& - \Fuu\inv \, \left[\Fux \,\dxvb - \muv - \diag(\pvt^{\rm max}_{\rm rel}(\omega))\, \gammav \right] \nonumber \\
\uvt &=& -\Futut\inv\, \left[ 
\Futxt \,\xvt -\diag\left(\frac{\uvt}{|\uvt|}\right))\, \gammav \right].
\end{eqnarray}

\subsection{Economic balance equation for enzyme rhythms, Eqs~(\ref{eq:EconomicBalanceStaticPeriodic}) and (\ref{eq:EconomicBalanceStaticPeriodic2})}
\label{sec:SIProofPeriodicbalanceequations}

We now derive economic balance
equations for periodic  states. We consider a state in which
rhythms $\xvt$ and $\uvt$ drive oscillations $\vvt$ and $\cvt$, and we 
study the effects of small additional enzyme variations ($\delta \uvb$
and $\delta \uvt$), whose effects on mass balances are compensated by
periodic exchange fluxes ($\delta \bar \varphiv, \delta \tilde
\varphiv)$. The compensation is chosen such that all metabolite
profiles remain unchanged: $\delta \cvb=0, \delta \cvt=0$. The fluxes,
however, will change: to compute the variations, $\vvb$ and $ \vvt$,
we expand them in terms of $\delta \uvb$ and $\delta \uvt$:
\begin{eqnarray}
{ \delta \vv \choose \delta \vvt} &=& \left(\begin{array}{ll}
  \Eper^{v}_{u} & \Eper^{v}_{\tilde u}\\ \Eper^{\tilde v}_{u} &
  \Eper^{\tilde v}_{\tilde u}\\\end{array} \right) { \delta \uv
    \choose \delta \uvt}.
\end{eqnarray}
The rhythmic elasticities $\Eper^{\rm x}_{\rm y}$ refer to the
periodic, unperturbed state (see \ref{sec:SIperiodicElasticities}).
 To compensate the effects of $\delta \uv$
and $\delta \uvt$ on all mass balances, the virtual fluxes must compensate 
the perturbed mass balances
$\Nint \, \delta \vv$ and $\Nint \, \delta \vvt$) and  must therefore read
\begin{eqnarray}
{ \delta \varphiv \choose    \delta \tilde \varphiv}
&=& - \left( \begin{array}{ll} \Nint & 0 \\ 0 & \Nint \end{array}\right)
{ \delta \vv \choose \delta \vvt}
= - \left( \begin{array}{ll} \Nint & 0 \\ 0 & \Nint \end{array}\right)
\left(\begin{array}{ll}
  \Eper^{v}_{u}      & \Eper^{v}_{\tilde u}\\
  \Eper^{\tilde v}_{u} & \Eper^{\tilde v}_{\tilde u}\\
\end{array} \right)
{ \delta \uv \choose    \delta \uvt}.
\end{eqnarray}
We now defined the static and periodic enzyme demands $\perguv$ and $\perguvt$
as derivatives between the {\metabolicobjective} functional and
enzyme variations.  The static or periodic economic
potentials $\perwrv$ and $\perwrvt$ can be  defined, in a very similar way, 
 as derivatives between
{\metabolicobjective} functional and virtual fluxes:
\begin{eqnarray}
  \perguv  &=& \frac{\partial g}{\partial \uv}, \qquad
  \perguvt  =  \frac{\partial g}{\partial \uvt}\nonumber \\
  \perwrv  &=& \frac{\partial g}{\partial \varphiv}, \qquad
  \perwrvt  =  \frac{\partial g}{\partial \tilde \varphiv}.
\end{eqnarray}
 The compensated variation results in a total {\metabolicobjective} change, which can be
expressed by the {\metabolicobjective} changes caused by the variations of enzyme
levels and virtual fluxes: 
\begin{eqnarray}
\label{eq:enzymevalue10}
  \delta g &=& \real\left[ {  
      \perguv}\trans\,\delta \uv
  +   \perwrvt^\dag\,\delta \uvt 
  +   \perwrv\,\delta  \varphiv 
  +   \perwrvt\,\delta \tilde \varphiv \right]
  \nonumber \\ &=& \real\left[ {\perguv \choose \perguvt }^\dag
            {\delta \uv \choose \delta \uvt} +{\perwrv \choose
              \perwrvt}^\dag {\delta \varphiv \choose
              \delta \tilde \varphiv} \right] \nonumber \\ 
            &=& \real\left[ { \perguv
              \choose {\perwrvt}}^\dag {\delta \uv \choose \delta \uvt}
            -{\perwrv \choose \perwrvt}^\dag
            \left(\begin{array}{ll} \Nint & 0 \\ 0 &
              \Nint \end{array}\right) \left(\begin{array}{ll}
              \Eper^{v}_{u} & \Eper^{v}_{\tilde u}\\ \Eper^{\tilde
                v}_{u} & \Eper^{\tilde v}_{\tilde u}\\
\end{array} \right)
{\delta \uv \choose \delta \uvt} \right].
\end{eqnarray}
The same {\metabolicobjective} change can also be written in terms of  local
flux variations (here metabolite variations  can be neglected because 
they are cancelled in  the compensated
variation):
\begin{eqnarray}
\label{eq:enzymevalue11}
  \delta g &=& \real\left[ {{\bvtot} \choose  {\bv_\vt}}
\cdot
{\delta  \vv  \choose \delta \vvt }
= {{\bvtot} \choose  {\bv_\vt}}^\dag
 \left(\begin{array}{ll}
   \Eper^{v}_{u} & \Eper^{v}_{\tilde u}\\ \Eper^{\tilde v}_{u} & \Eper^{\tilde v}_{\tilde u}\\
\end{array} \right)
{\delta \uv \choose \delta \uvt} \right].
\end{eqnarray} 
We now equate Eqs (\ref{eq:enzymevalue10}) and
(\ref{eq:enzymevalue11}). Since the equality must hold for any choice
of the vector ${\delta \uv \choose \delta \uvt}$, we obtain the
economic rule
\begin{eqnarray}
  {\perguv \choose \perguvt } 
  &=&  
  \left(\begin{array}{ll}
    \Eper^{v}_{u}      & \Eper^{v}_{\tilde u}\\
    \Eper^{\tilde v}_{u} & \Eper^{\tilde v}_{\tilde u}\\
  \end{array} \right)^\dag
  {{\Nint}\trans \perwrv + \bvtot\choose  {\Nint}\trans \perwrvt +  {\bv_\vt}},
\end{eqnarray}
which links  enzyme demands, economic potentials, and flux gains.  Noting
that ${\Nint}\trans \wrv = \Deltar\wrv$ and equating the enzyme
demands to the {\price}s $\perhuv$ and $ \perhuvt$, we obtain the
economic balance equation
\begin{eqnarray}
\label{eq:SIEconomicBalanceEquations0}
  {\perhuv \choose \perhuvt } 
  &=&  
  {\perguv \choose \perguvt } 
  =
  \left(\begin{array}{ll}
    \Eper^{v}_{u}      & \Eper^{v}_{\tilde u}\\
    \Eper^{\tilde v}_{u} & \Eper^{\tilde v}_{\tilde u}\\
  \end{array} \right)^\dag
  {\Deltar \perwrv + \bvtot\choose  \Deltar \perwrvt +  {\bv_\vt}}.
\end{eqnarray}
This balance equation holds generally even far from steady state.
 If our periodic state is close
to a steady reference state, we can  expand the effective
elasticities, use Eq.~(\ref{eq:effectivePeriodicEnzymeElasticities}) from
section \ref{sec:SIproofperiodicElasticities}, and obtain 
\begin{eqnarray}
\label{eq:SIEconomicBalanceEquations1}
  {\diag(\uv)\,\perhuv \choose \diag(\uv)\,\perhuvt } 
  &=&  
  {\diag(\uv)\,\perguv \choose \diag(\uv)\,\perguvt } 
  =
\left(\begin{array}{lr}
\diag(\mathring{\vvb}) & \diag(\mathring{\vvt}) \\
\diag(\mathring{\vvt}) & \diag(\mathring{\vvb})
\end{array} \right)
^\dag
  {\Deltar \perwrv + \bvtot\choose  \Deltar \perwrvt +  {\bv_\vt}},
\end{eqnarray}
where $\mathring{\vvb}$ and $\uv$ are the vectors of fluxes and enzyme
levels in the central state, and we defined $\mathring{\vvt} =
\Emat^{\rm v}_{\rm c}\, \cvt + \Emat^{\rm v}_{\rm x}\,\xvt$.

}

\begin{table*}[t!]
\begin{center}
\begin{tabular}{|lll|}
\hline 
  \rowcolor{cbatablecolor1} 
  \textbf{Symbol} & \textbf{Unit} & \textbf{Name} \\
  \hline
  $\cint_{i}$   & mM &Concentration  \\
  $v_{l} = \rate_{l}(\u_l,\cintv)$   & mM/s &Reaction rate \\
  $\ratelaw_{l}(\u_l,\cintv)$   & mM/s &Catalytic rate\\
  $\u_{l}$  & mM &enzyme activity \\
  $\x_{j}$  &  &External parameter \\
  $p_{m}$   & & State parameter (enzyme activity or external parameter) \\\hline
  $\csteady_{i}$   & mM &Steady state concentration \\
  $\vsteady_{l}$   & mM/s &Steady state flux (reaction rate) \\
  $\ffit(\uv)$       & D &Fitness function: $\ffit(\uv)= \gplus(\uv)- \hminus(\uv)$\\
  $\gplus(\uv) = \yy(\vv(\uv),\cintv(\uv))$       & D & {\metabolicobjective} function  \\
  $\hminus(\uv)$       & D & {\Investment} function \\
  $\yy^{\rm v}_{l}$   & D/(mM/s) & \co{FIX mE!} Flux {\gain} $\yy^{\rm v}_{l} = \partial \yy/\partial v_l$\\
  $\omega$ & s$\inv$ & Circular frequency\\ \hline
  $\Ffunctional^{\rm (S)} = \ffit(\langle \ysv(t) \rangle_t)$ & D$\inv$ & State-average fitness functional \\ 
  $\Ffunctional^{\rm (F)} = \langle \ffit(\ysv(t)) \rangle_t$ & D$\inv$ & Fitness-average fitness functional \\ \hline
 $\Imat$ & & Identity matrix \\
  \hline
\end{tabular}
\end{center}
\caption{Mathematical symbols used. \co{schoenere symbole statt FS und FFß} 
  The biological meaning of the parameters $\u_l$ and $\x_l$, as well as
  their physical units, can vary from case to case.  The hypothetical unit Dw
  (Darwin) stands for whatever fitness unit is used in a model.}
\label{tab:symbols}
\end{table*}

\section{Mathematical notation for metabolic oscillations}
\label{sec:SInotation}

\myparagraph{\ \\Complex vectors and matrices} \co{The scalar product
  between complex-valued vectors is defined as
  $\av \cdot \bv = \real[\av^\dag \,\bv]$.}  The formulae in the
article are written in matrix notation, with vectors, matrices, and
tensors written in bold font. By default, all vectors are column
vectors. The adjoint $\zv^\dag$ of a complex vector $\zv$ is defined
as the complex conjugate transpose $\zv^\dag = (z_1^*, .., z_n^*)$
(i.e.~a row vector, where the star * indicates the complex conjugate).
For convenience, we define a scalar product
$\av\cdot \bv = \av^\dag\,\bv$ for complex vectors. If a real-valued
result is required, this must be stated explicitly as
$\real(\av\cdot \bv)$.  We can use the formula
$\real(\av\cdot \bv) = \real(\av)\cdot\real(\bv) +
\im(\av)\cdot\im(\bv)$ (with simple scalar products between
real-valued vectors on the right). The scalar product between a vector
and itself, $\av\cdot \av = \av^\dag\,\av$, yields a positive
real-valued number. Quadratic forms for complex vectors are written as
$\av^\dag\,\Mmat\,\bv$. If a matrix $\Mmat$ is self-adjoined
(i.e.~Hermitian), the quadratic form $\av^\dag\,\Mmat\,\av$ yields a
real-valued number.  Tensor products
$Y^{i}_{mn} = \sum_{l} A^{i}_{l} B^{l}_{mn}$ are written as
$\Ymat = \Amat \cdot \Bmat$; products
$X^{i}_{mn} = \sum_{pq} A^{i}_{pq} B^{p*}_{m} C^{q}_{n}$ are written
as $\Xmat = \Amat\, [\Bmat \otimes \Cmat]$. The symbol $\otimes$
denotes the Kronecker product.

\myparagraph{Complex amplitudes and complex derivatives} Oscillations are
described by the real parts of complex exponentials, for instance
$a(t) = \real(\e^{i \omega t}\,\at) = |\at| \cos(\omega t +
\varphi(\at))$,
where $\varphi(z)$ denotes the phase angle of a complex number
$z$. Oscillating vectors are written as
$\av(t) = \real( \tilde{\e^{i \omega t}\,\av}) = |\at_l| \cos(\omega t
+ \varphi(\at_l))$.
Note that amplitudes and amplitude vectors, marked by a tilde, are
complex-valued.  Complex derivatives are written as follows.  Let
$f(\zv)$ be a function of a complex vector $\zv$.  The first
derivative is represented by a column vector
$\fv_{\rm z} = \frac{\partial f}{\partial \zv} = (\frac{\partial
  f}{\partial z_1}, .., \frac{\partial f}{\partial z_n})\trans$,
where the complex derivatives of vector components
$z_l = x_l + i\,y_l$ are defined by
$\frac{\partial f}{\partial z_l}=\frac{\partial f}{\partial x_l} +
i\,\frac{\partial f}{\partial y_l}$.
For complex vectors $\av$ and $\bv$, we obtain the formula
$\frac{\partial}{\partial \bv} \real(\av \cdot \bv) = \av$. The second
derivatives of a function $f$ form a matrix $\Fmat_{\rm zz}$ with
elements
$F_{z_lz_k} = (\frac{\partial^2 f}{\partial z_l\,\partial z_k^*})$. As
an alternative notation, commonly used in metabolic control theory,
I also write this matrix as $\Dmat^f_{\rm zz}$, where $\Dmat$ can
stand for $\Emat$ (elasticity matrices) or $\Rmat$ (response
coefficient matrices).  If a function $f(\zv)$ of complex variables
can be Taylor-expanded, the second-order expansion reads
$f(\zv) \approx f(0) + \fv_{\rm z} \cdot \zv + \half \,\zv^\dag\,
\Fmat_{\rm zz}\,\zv$.
For real-valued functions $f$, the real part needs to be taken, so we
obtain
$f(\zv) \approx f(0) + \real(\fv_{\rm z} \cdot \zv) + \half
\,\zv^\dag\, \Fmat_{\rm zz}\,\zv$.

\begin{table*}[t!]
\begin{center}
\begin{tabular}{|ll|}
  \rowcolor{cbatablecolor1} 
\hline
\textbf{Steady states} & \\ \hline
  $\RYpmat = (\RYlpm)$ & 1$^{\rm st}$ order response coefficients for a state variable $\ys$\\
  $\RYppsecmat = (\RYlppsecmatmn)$ & 2$^{\rm nd}$ order response tensor (``synergy tensor'')  \\
  $\CSmat$,   $\CJmat$  &  Control coefficients for concentrations and fluxes\\
  $\epsilonSmat = (E_{li})$ & Unscaled elasticity matrix \\
  $\epsilonSSmat$,   $\epsilonSPmat$, 
  $\epsilonPSmat$,   $\epsilonPPmat$ & 2$^{\rm nd}$ order elasticity tensors \\ 
$\Fxu$,   $\Fuu$ & Static  fitness synergy matrices (Hessian matrices with respect to  $\duvb$ and $\Delta \xvb$)\\
\hline
\hline
 \rowcolor{cbatablecolor1} 
 \textbf{Periodic states} & \\\hline
  $\CSmat(\omega)$,   $\CJmat(\omega)$ & Spectral control coefficients for concentrations and fluxes\\
  $\RspecYpmat(\omega)      $ & 1$^{\rm st}$ order spectral response matrix \\
  $\RspecYbppsecmat(\omega) $, $\RspecYtppsecmat(\omega) $ & 2$^{\rm nd}$ order spectral response tensor for output $y$ at frequencies 0 and $2\,\omega$ \\
  $\RYbppsecmat(\omega)$,   $\RYtppsecmat(\omega)$ & 2$^{\rm nd}$ order periodic response tensor for output $y$ at frequencies  0 and $2\,\omega$\\
$\Fxtut$,   $\Futut$ & Periodic fitness synergy matrices (Hessian matrices with respect to  $\uvt$ and $\xvt$)\\\hline
\end{tabular}
\end{center}
\caption{Symbols for metabolic control theory. Unscaled
  {\MCA} coefficients (elasticities, response and control coefficients)
  are used throughout the text.}
\label{tab:symbols2}
\end{table*}
